# Supplementary material for: Transport Dependency: Optimal Transport Based Dependency Measures
Source: arXiv:2105.02073 source file (2023-03-20)

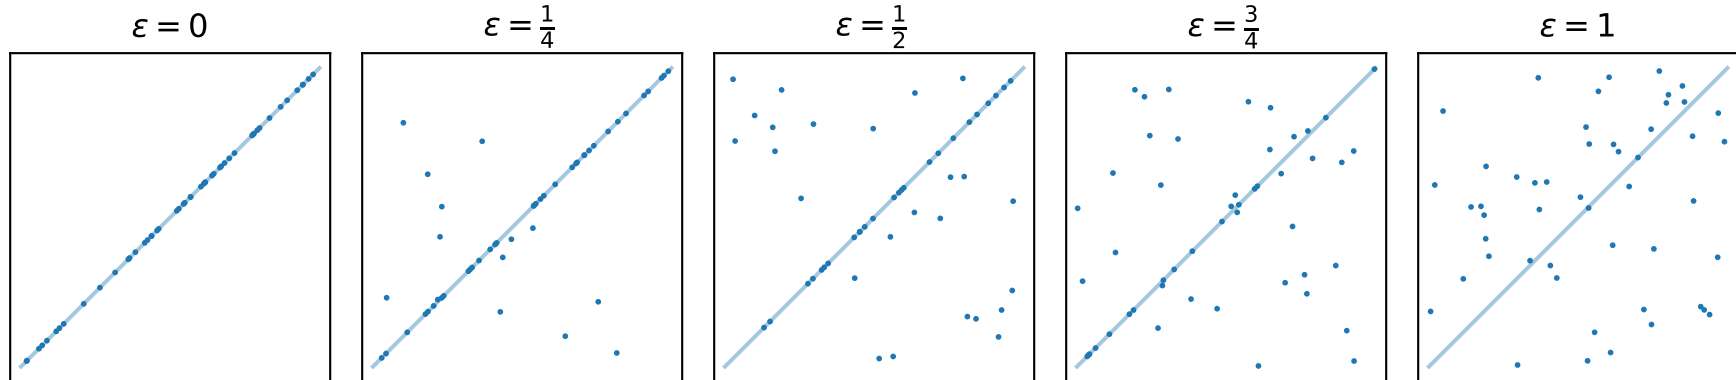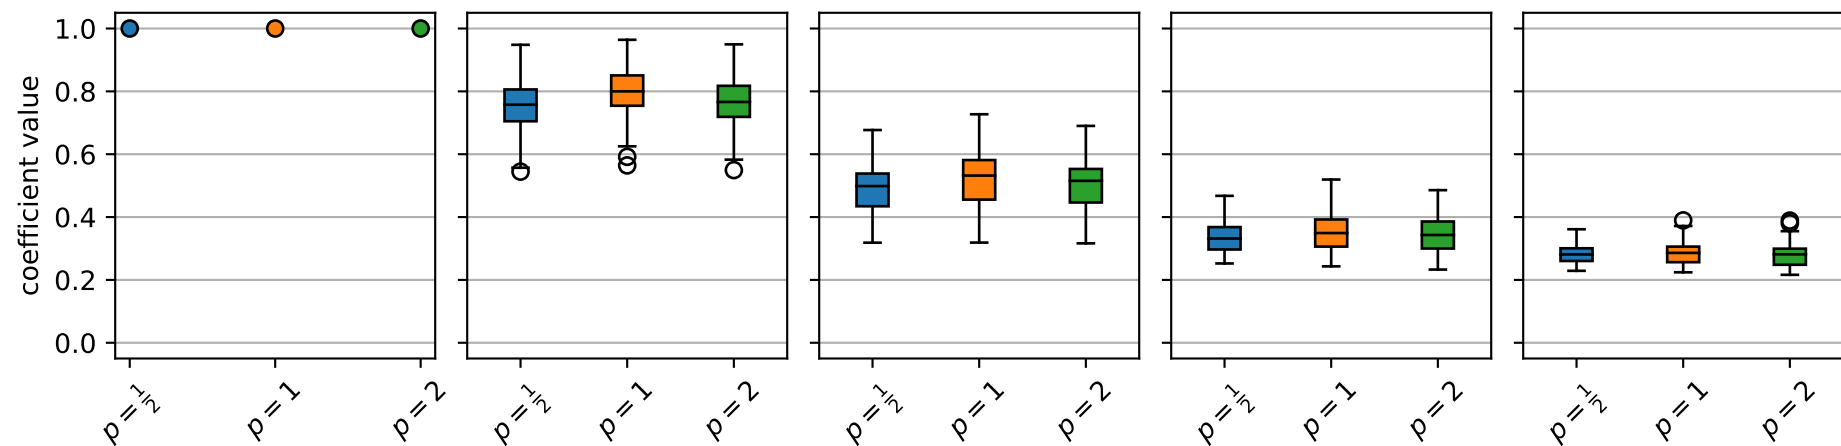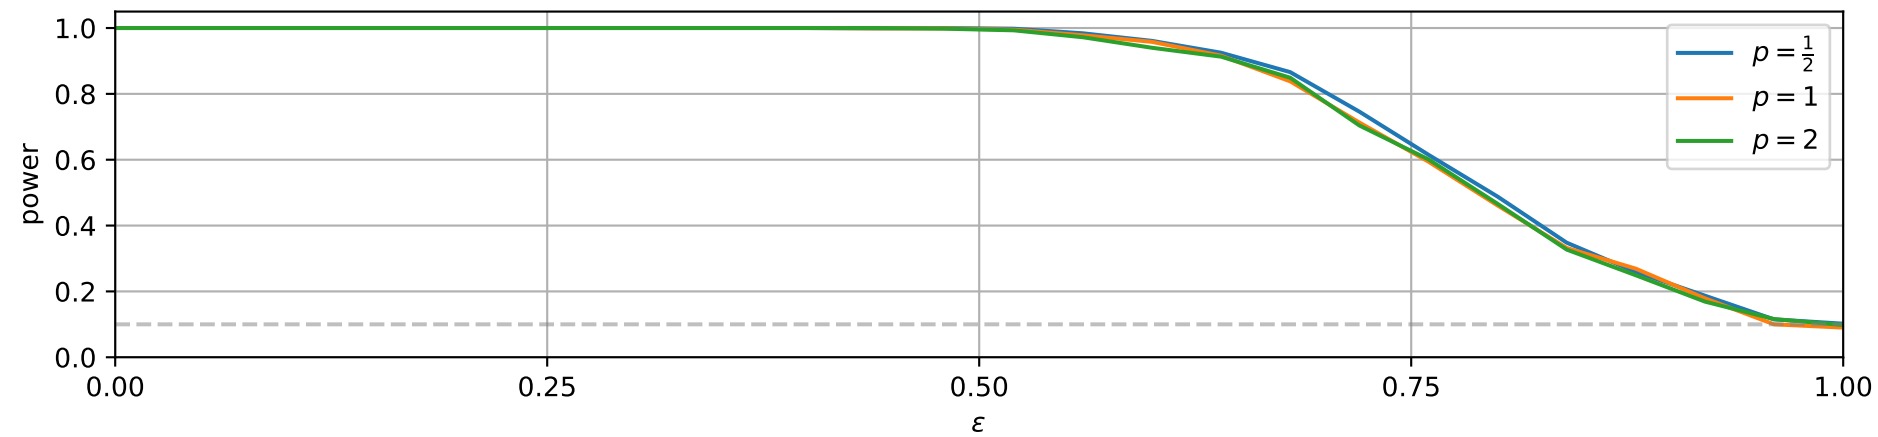

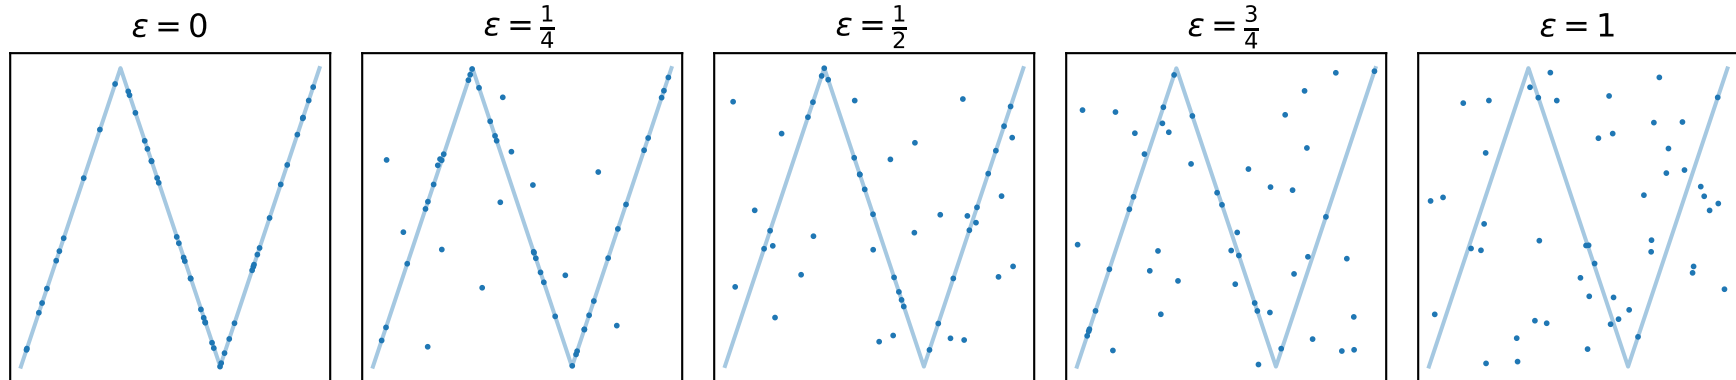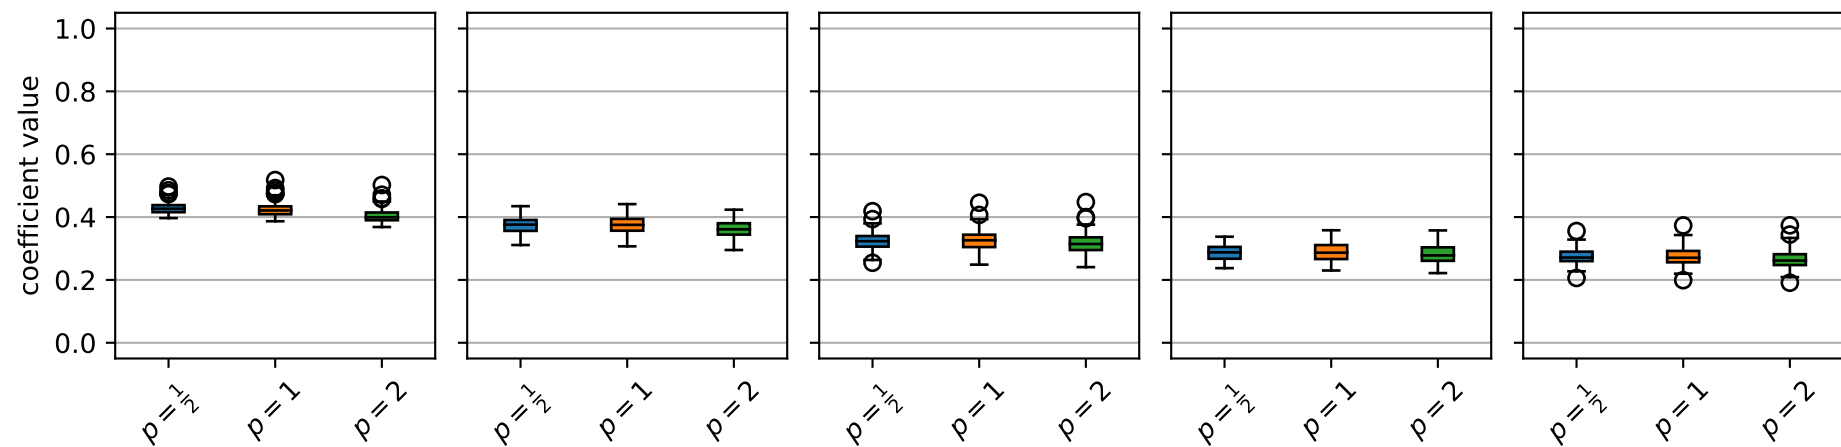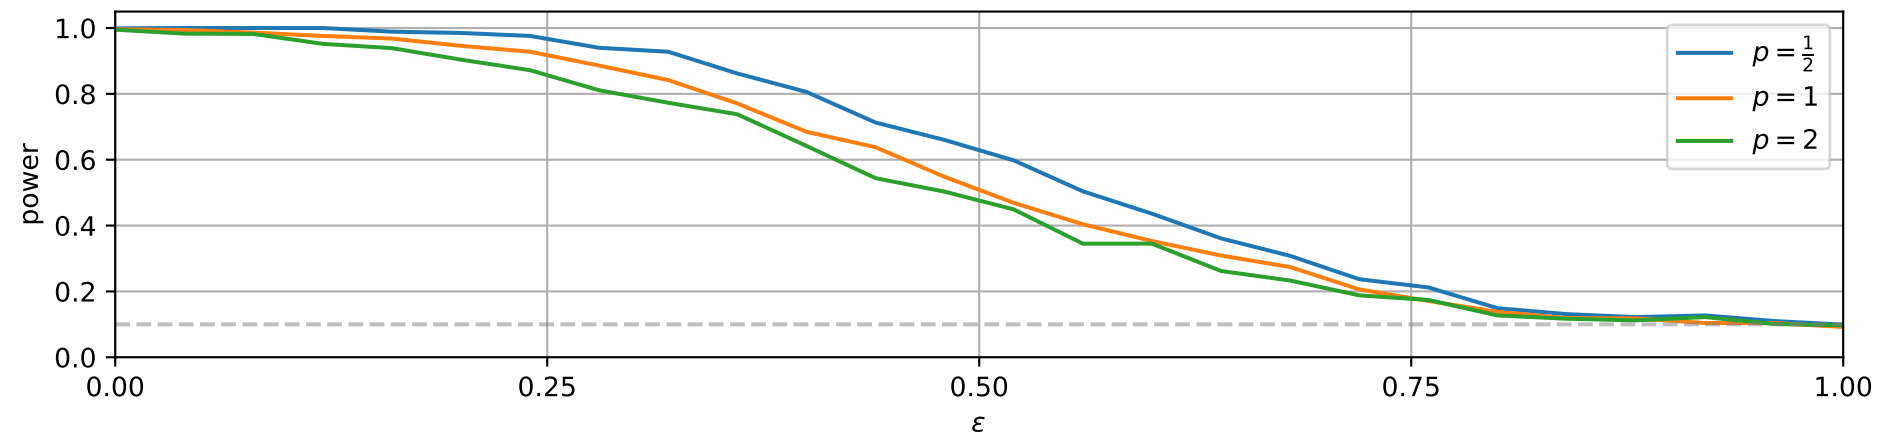

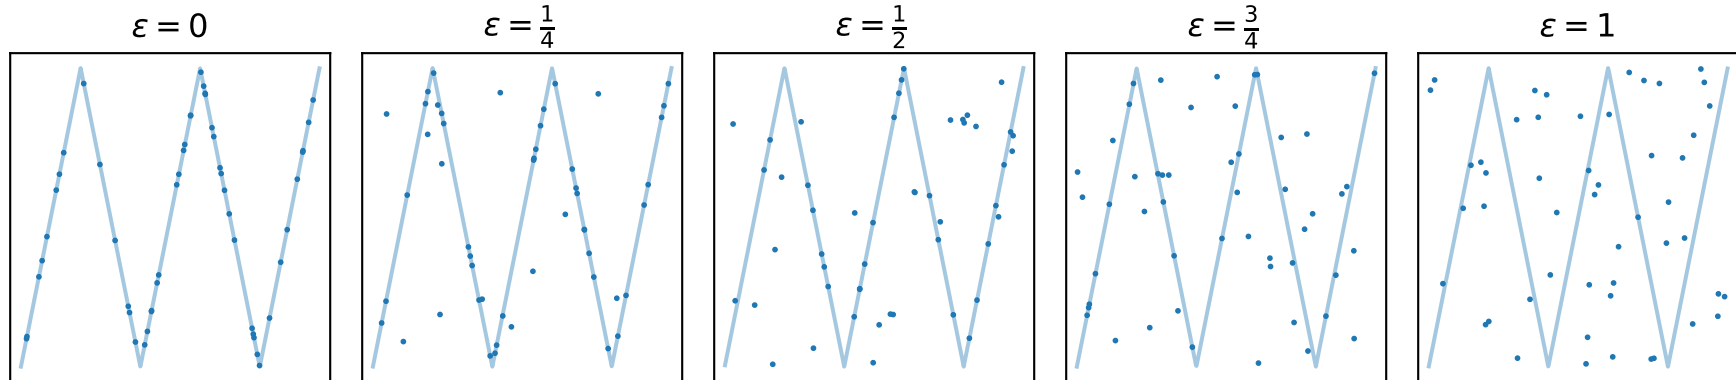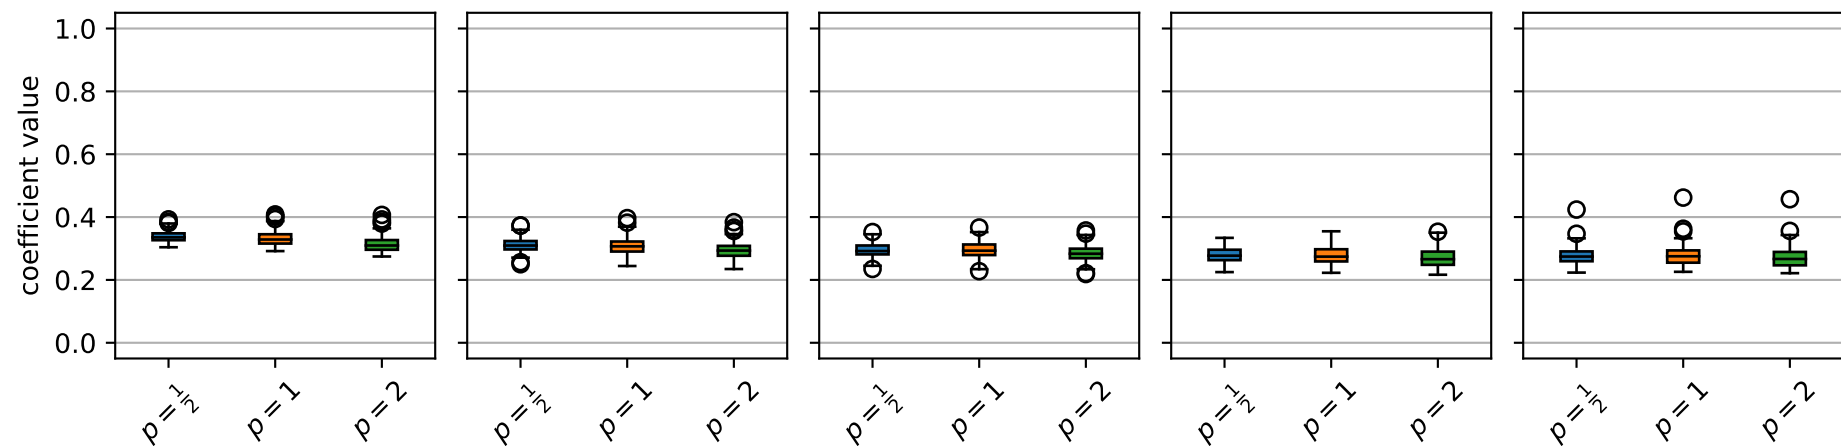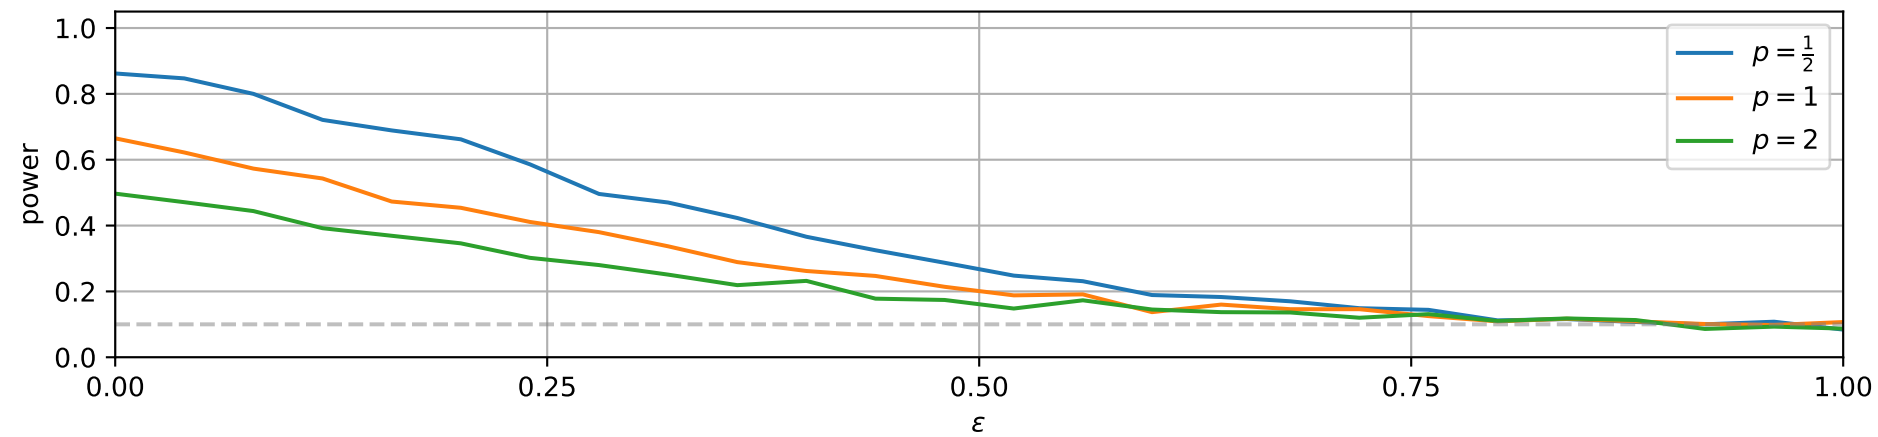

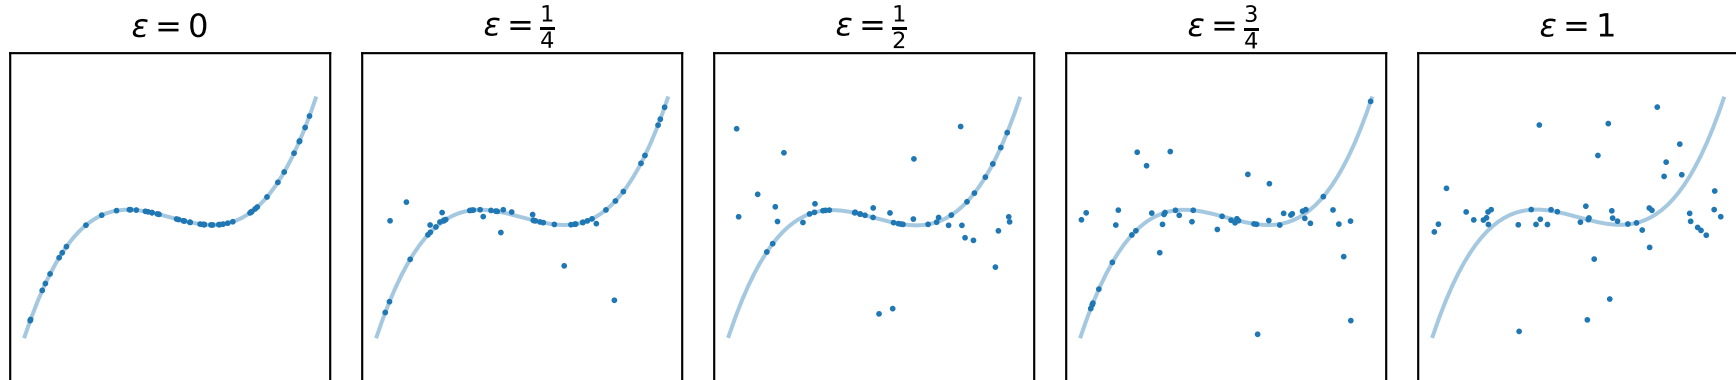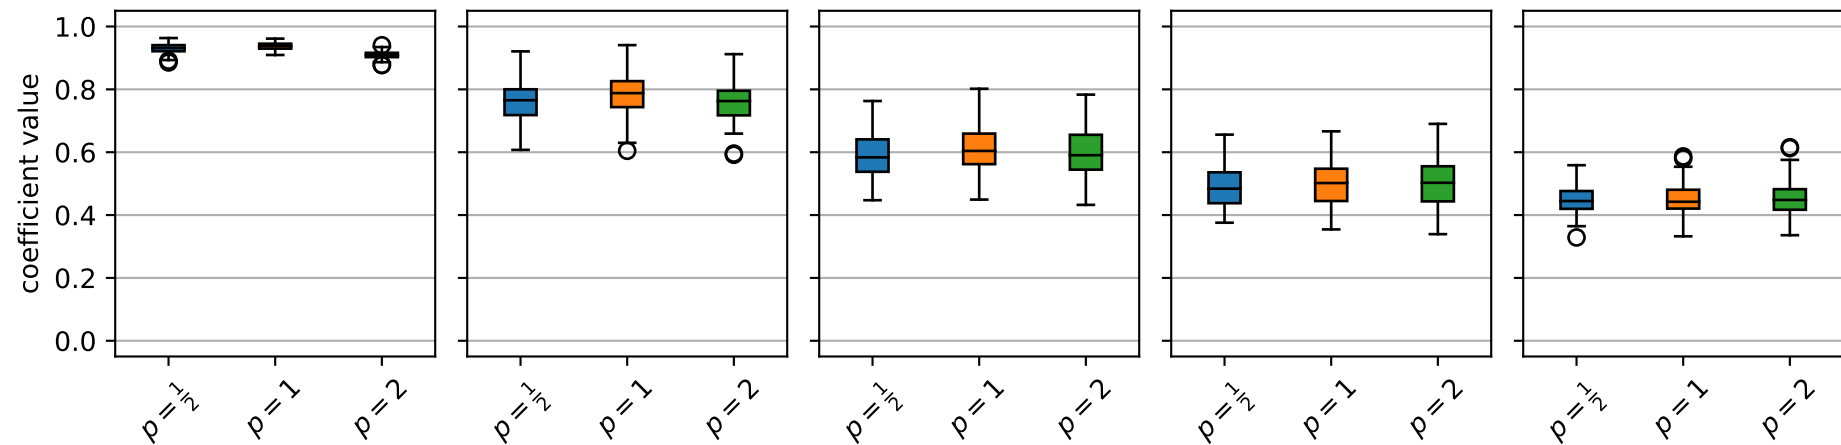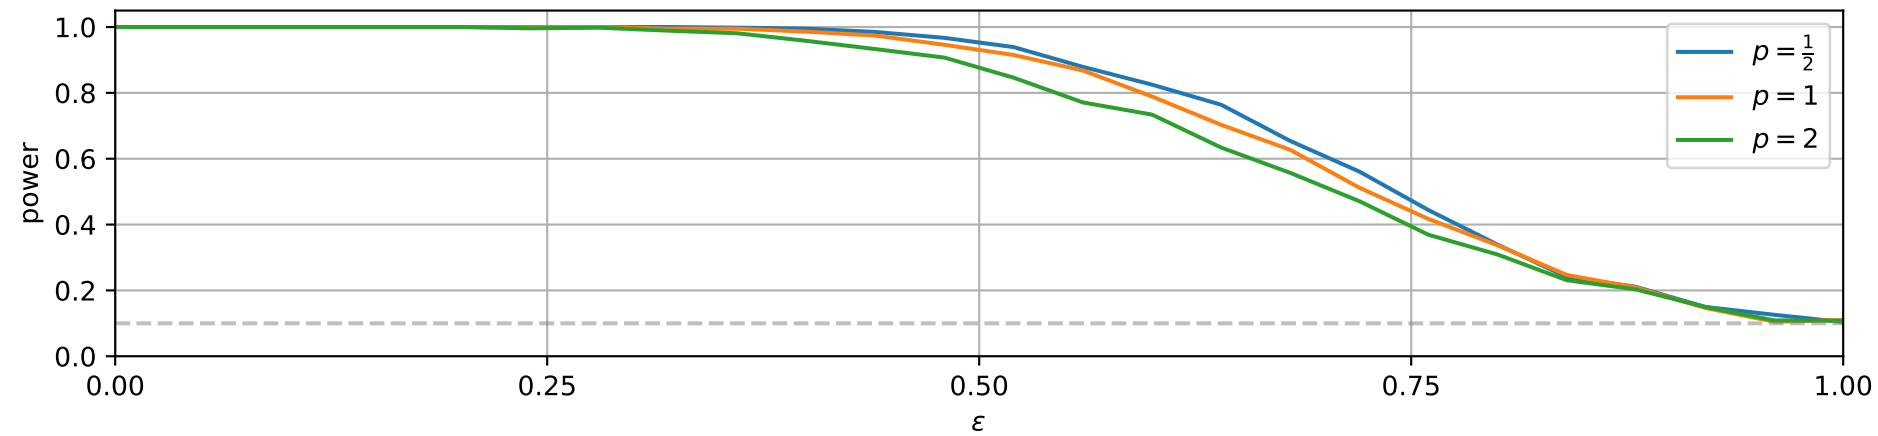

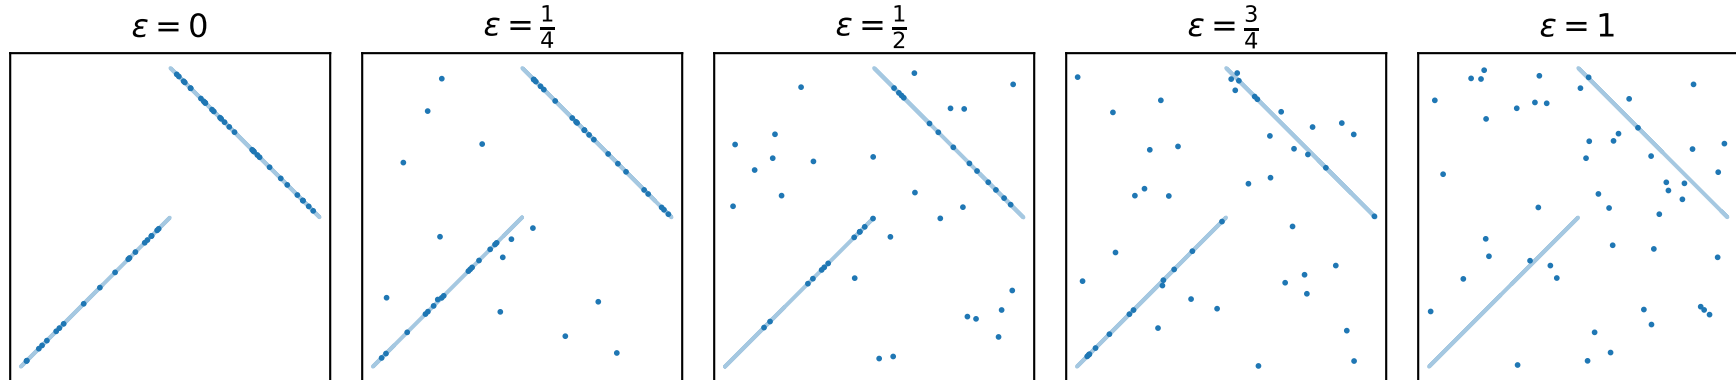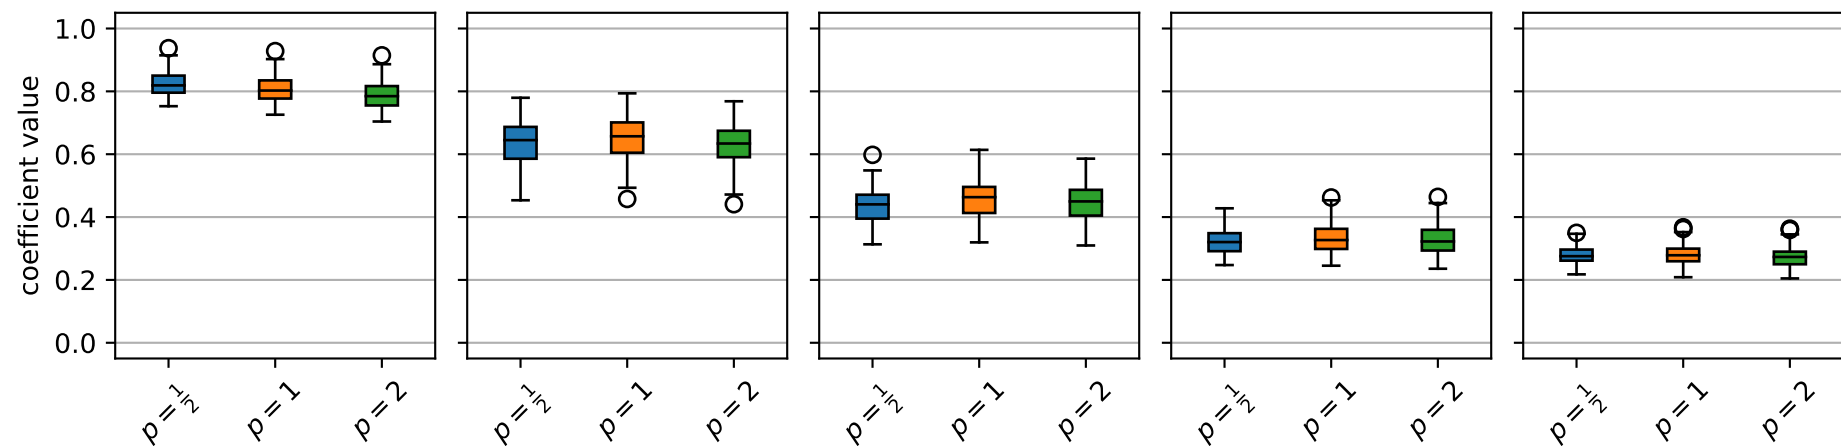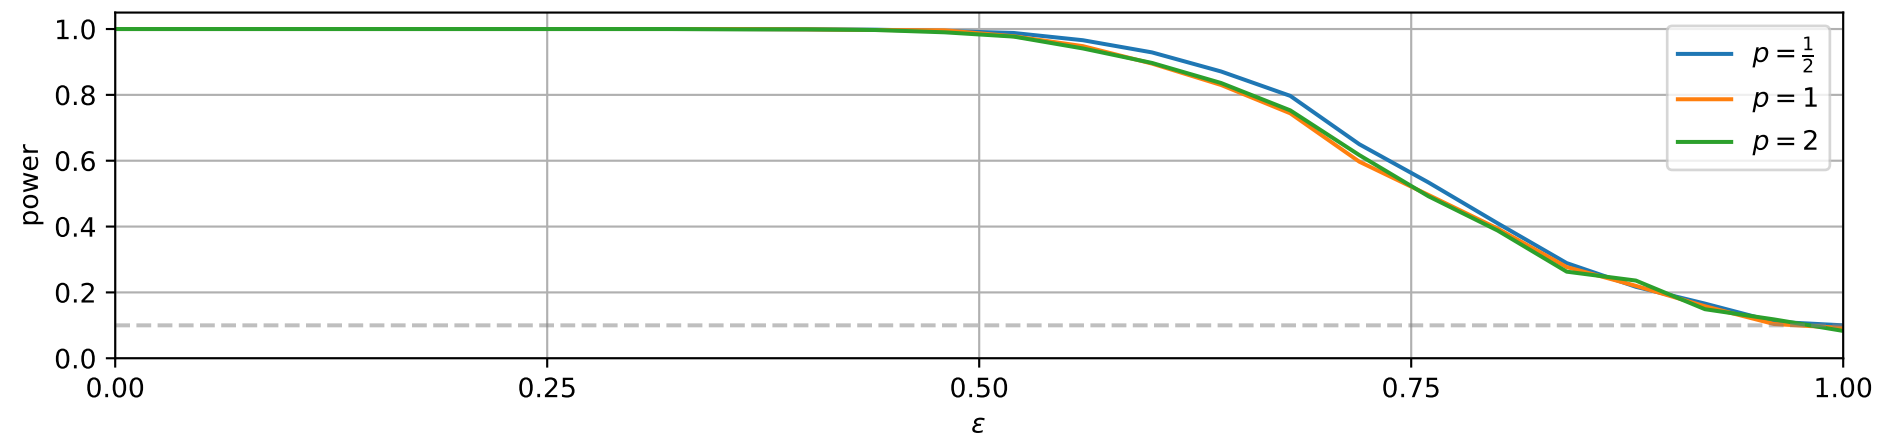

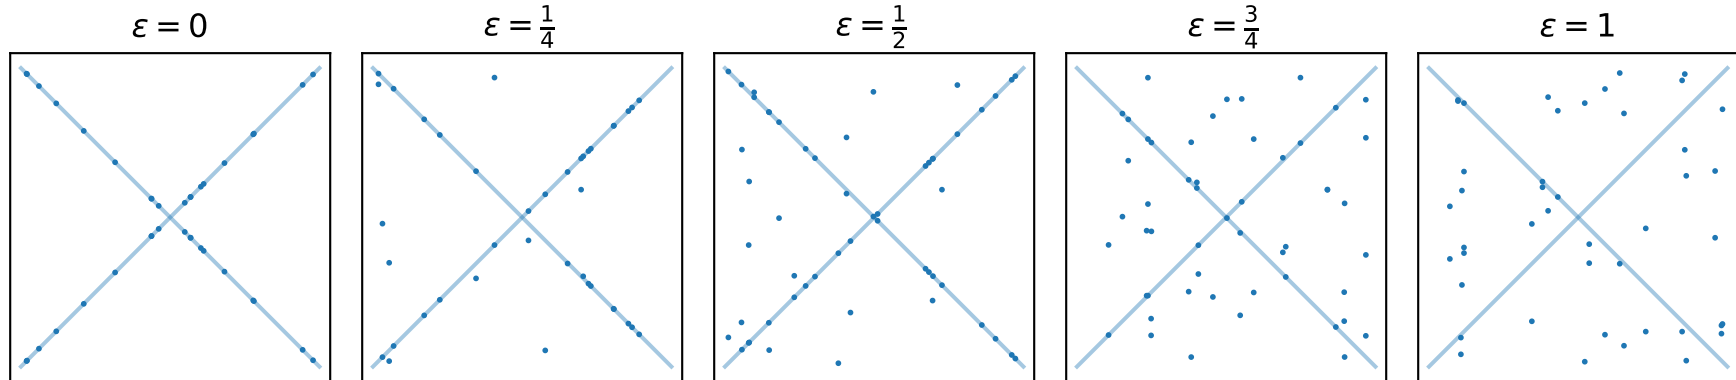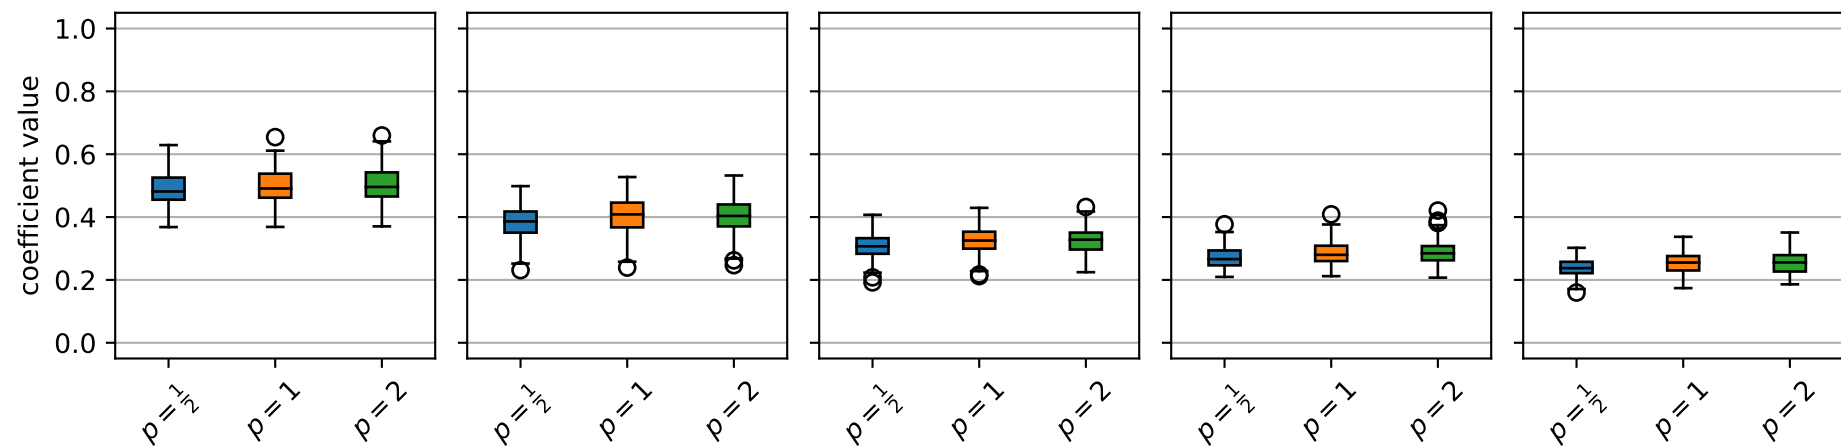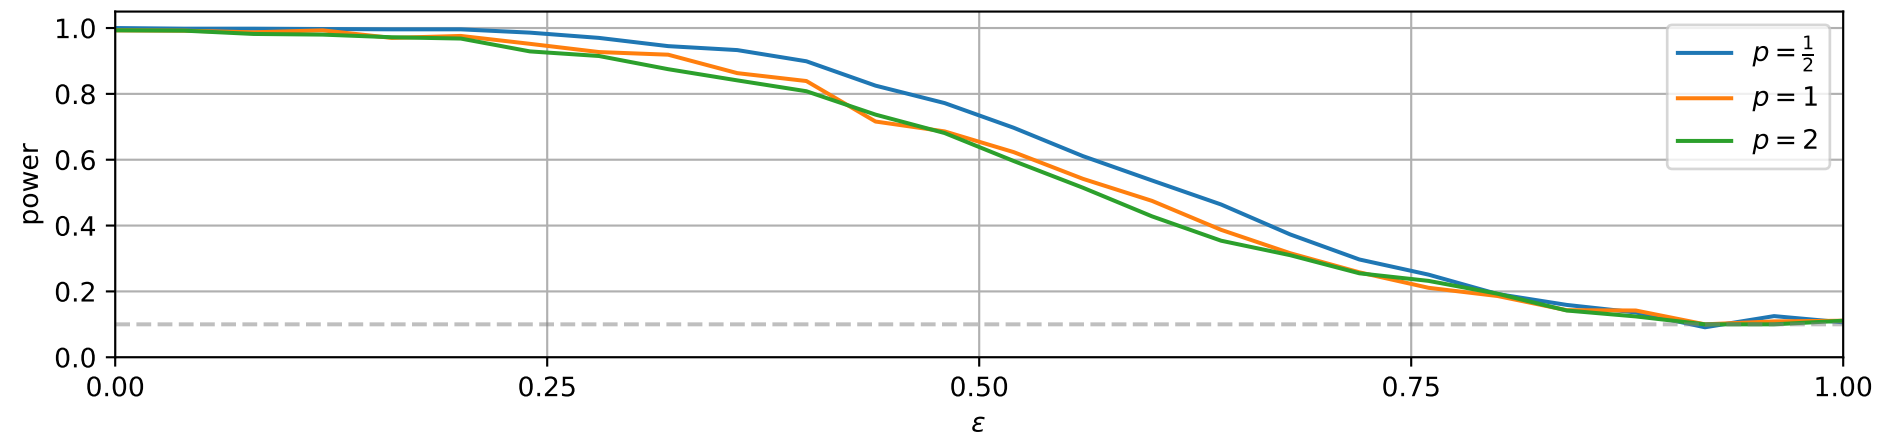

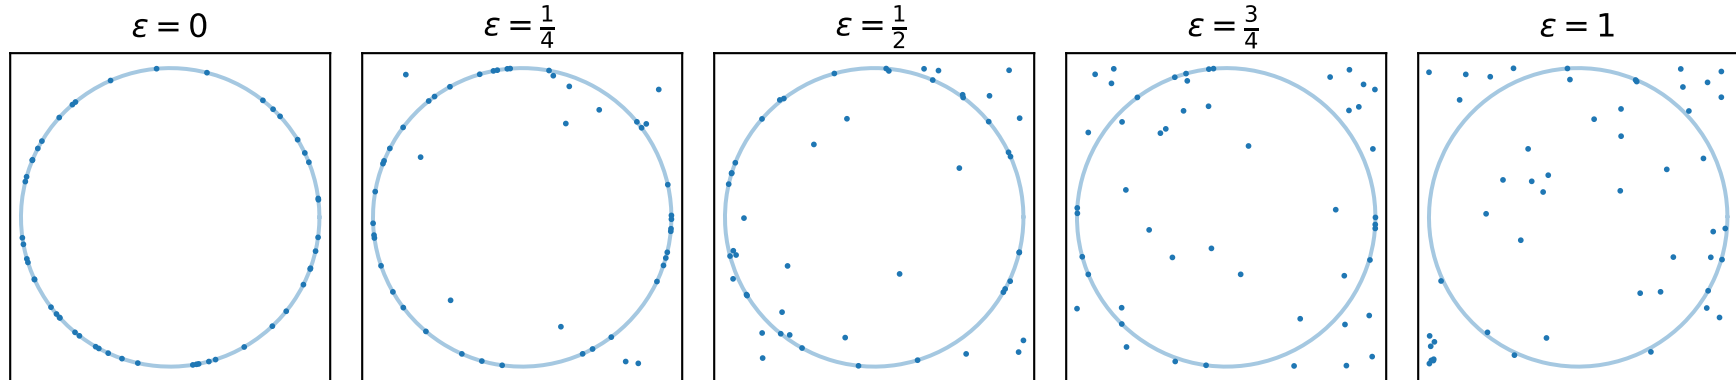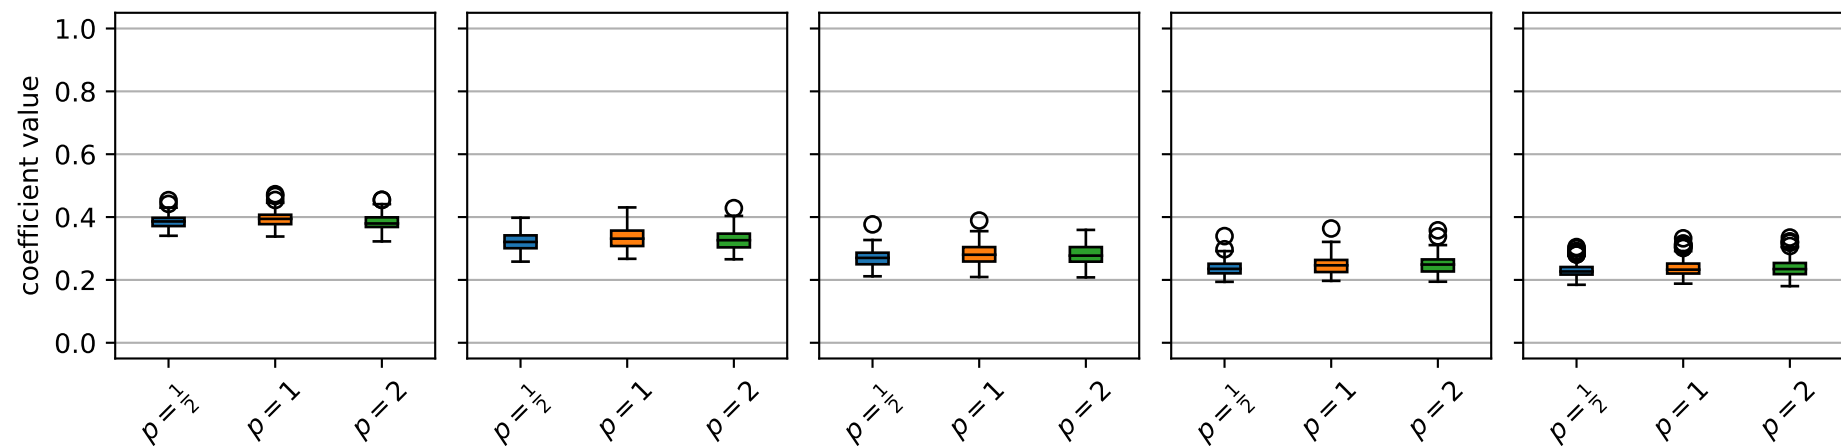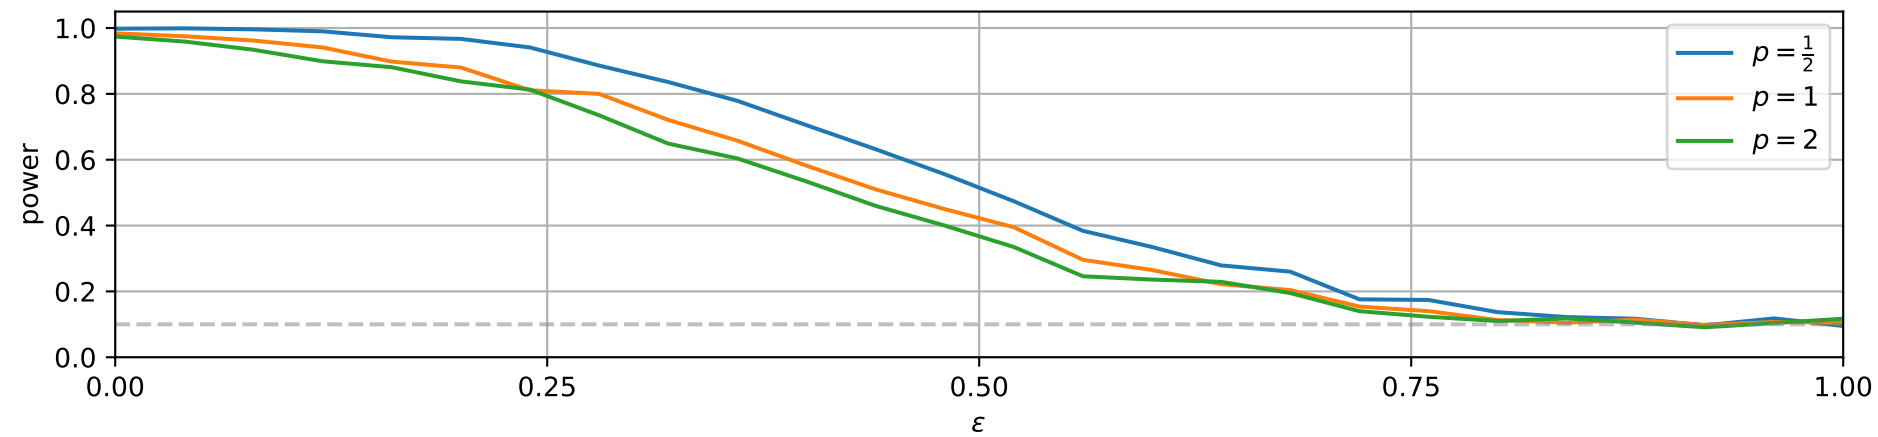

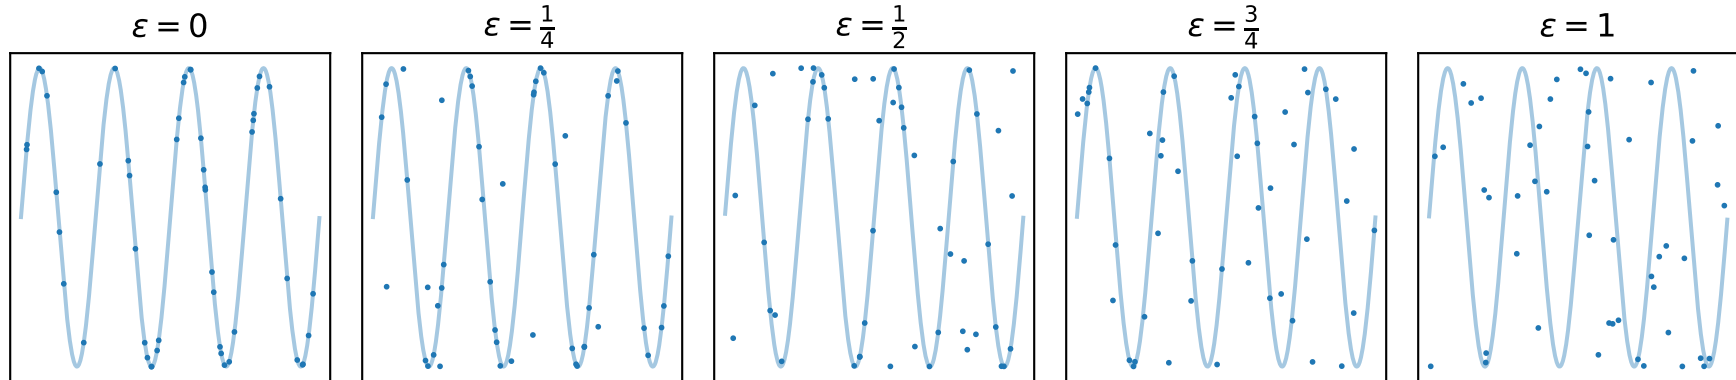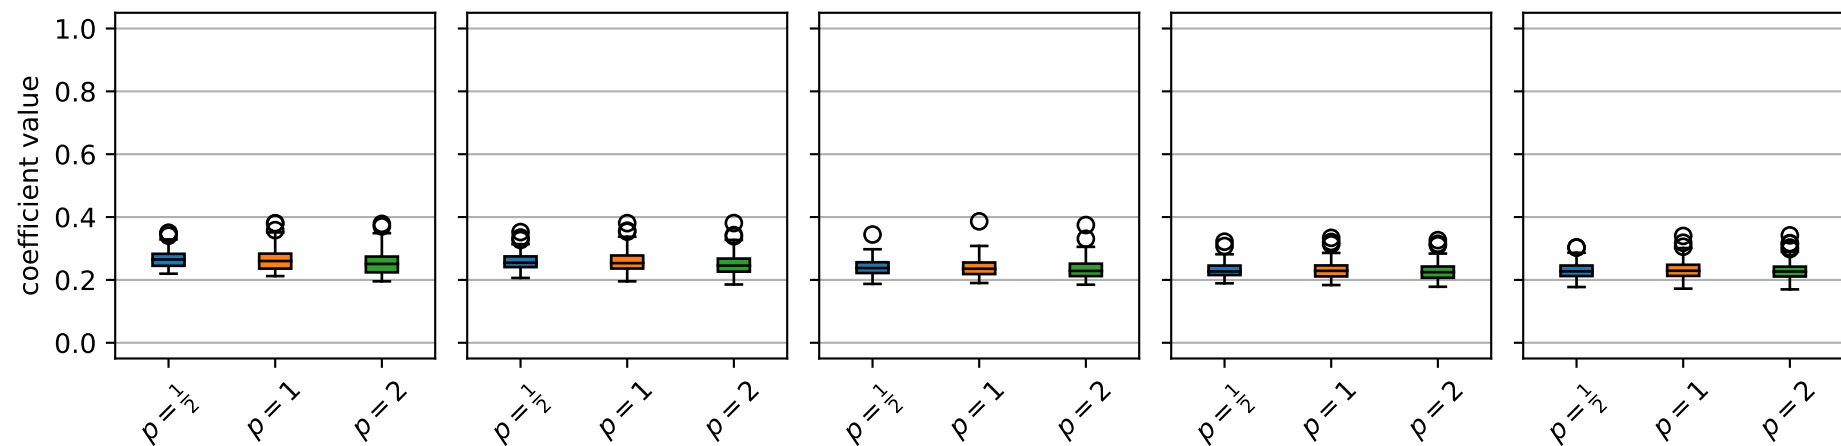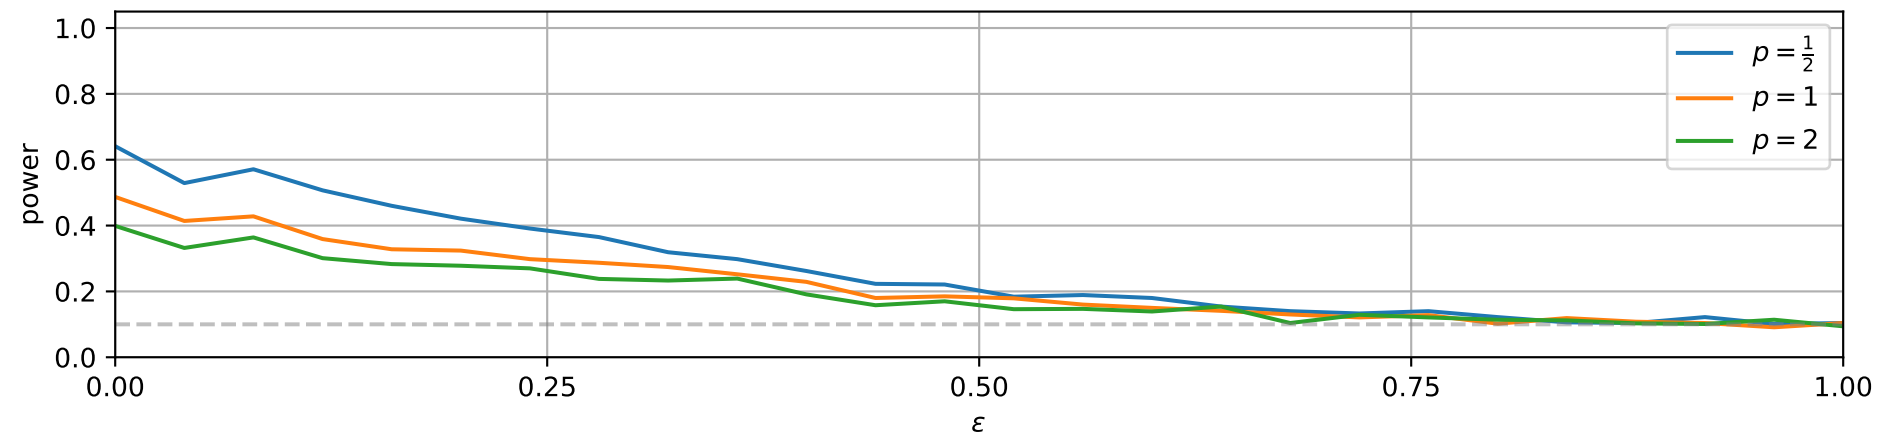



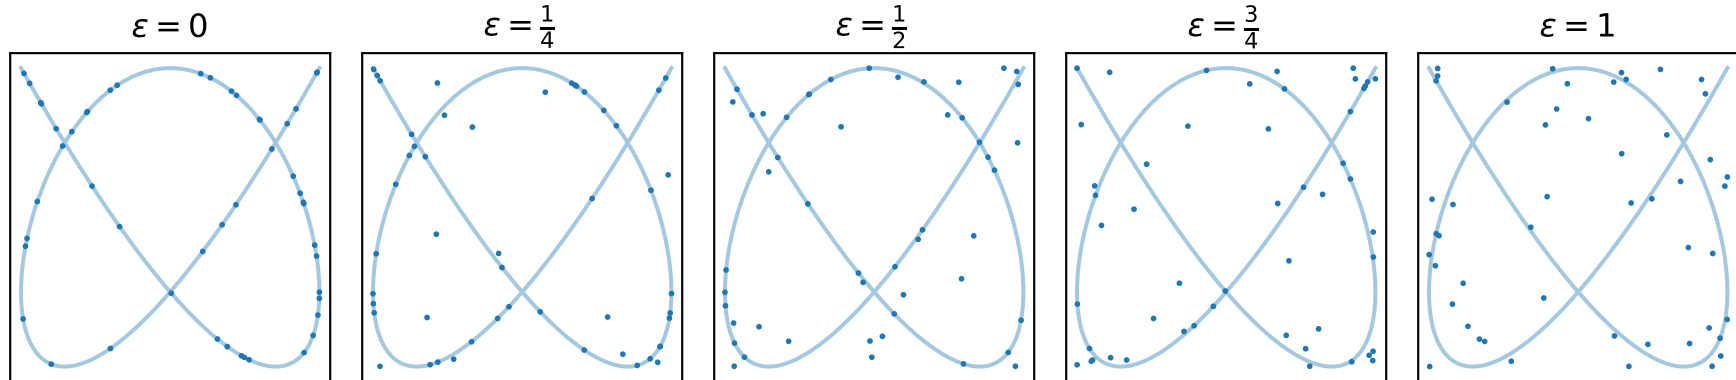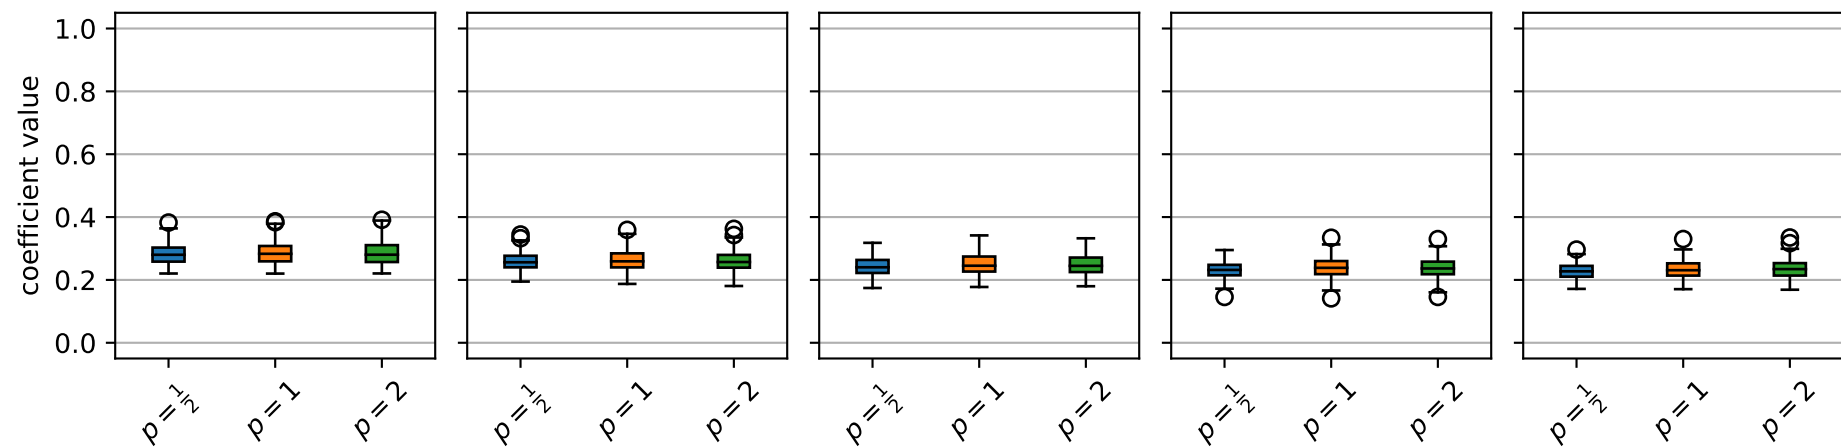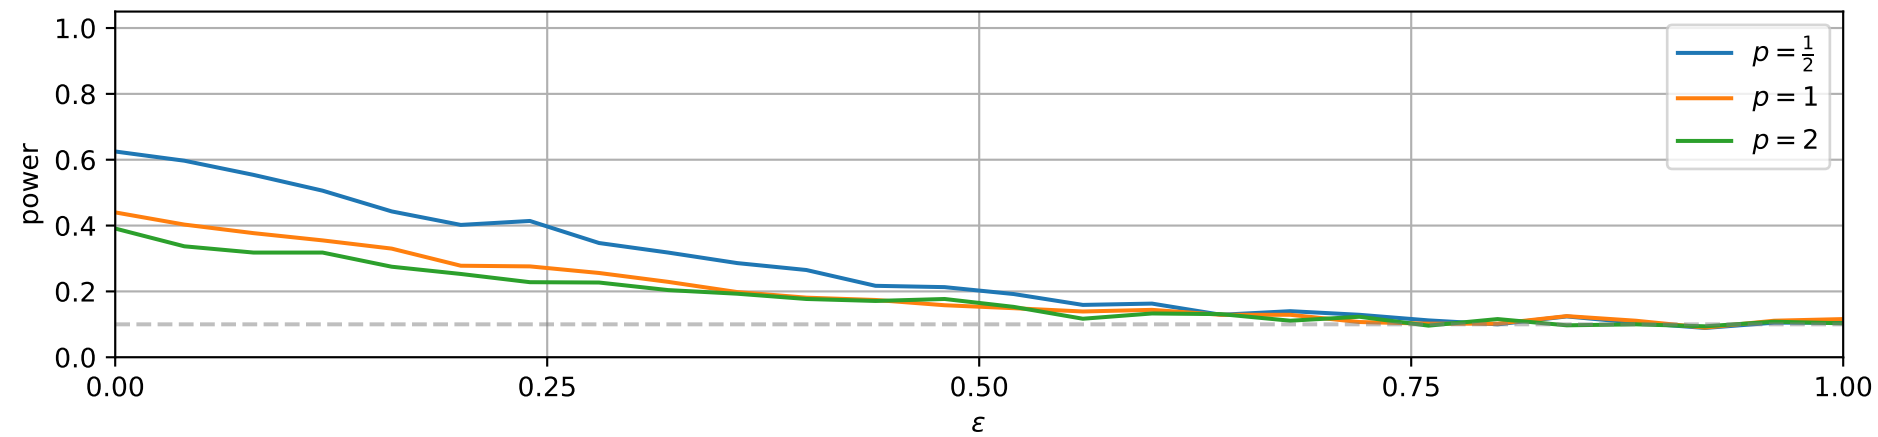

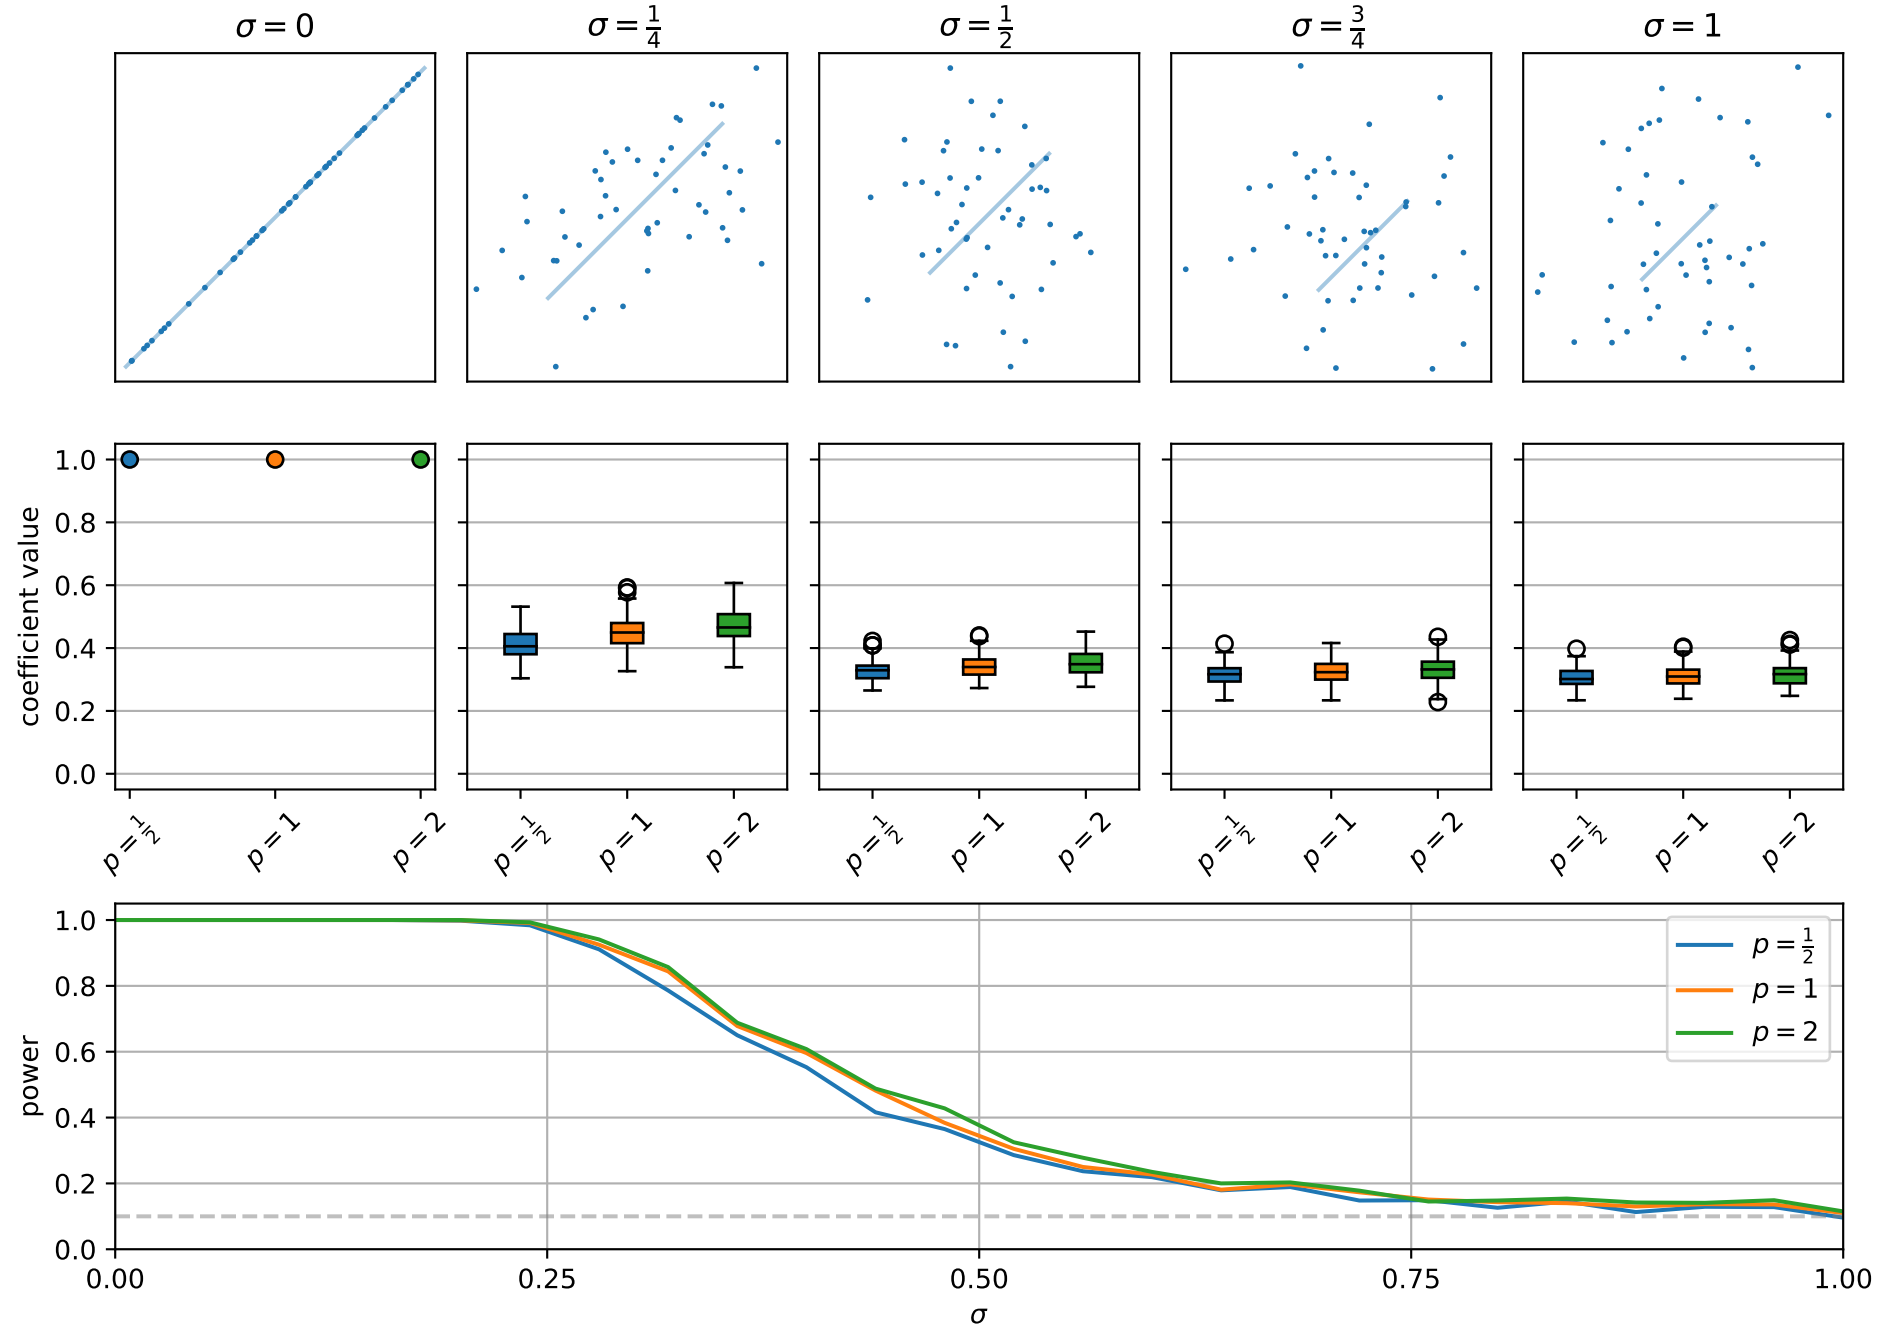

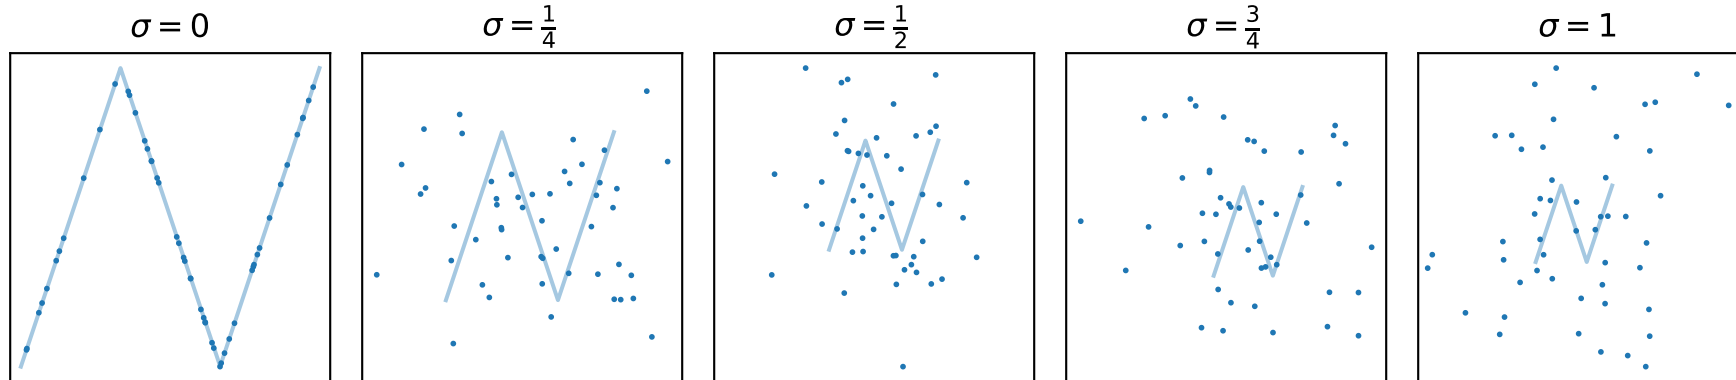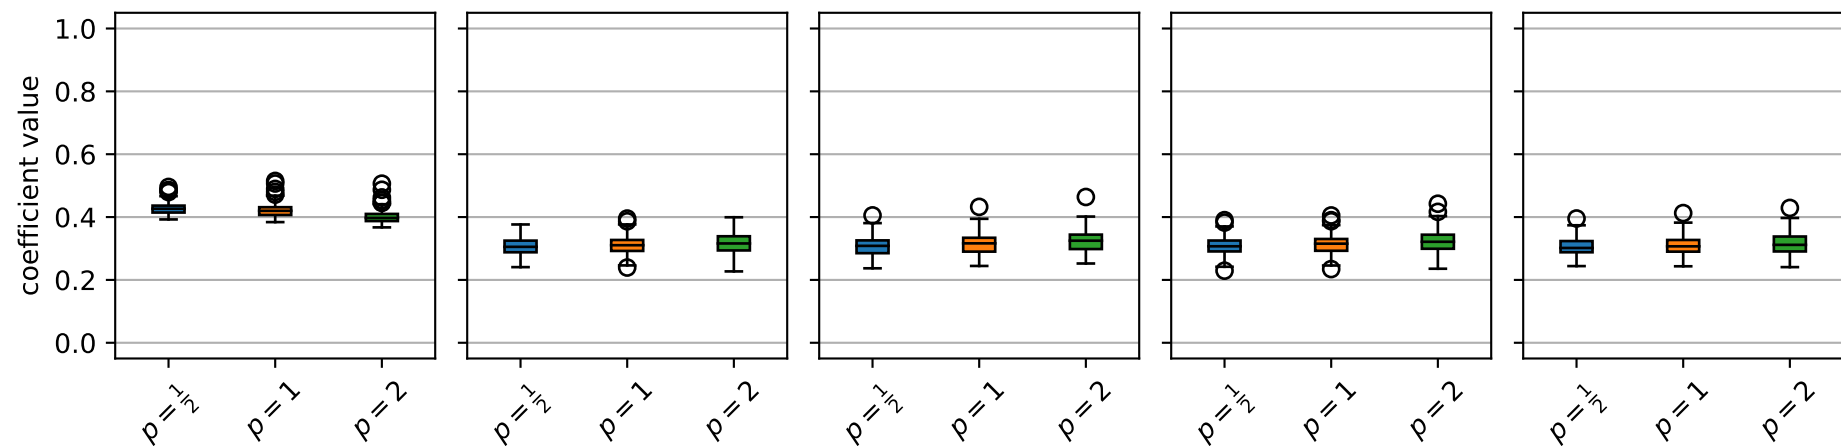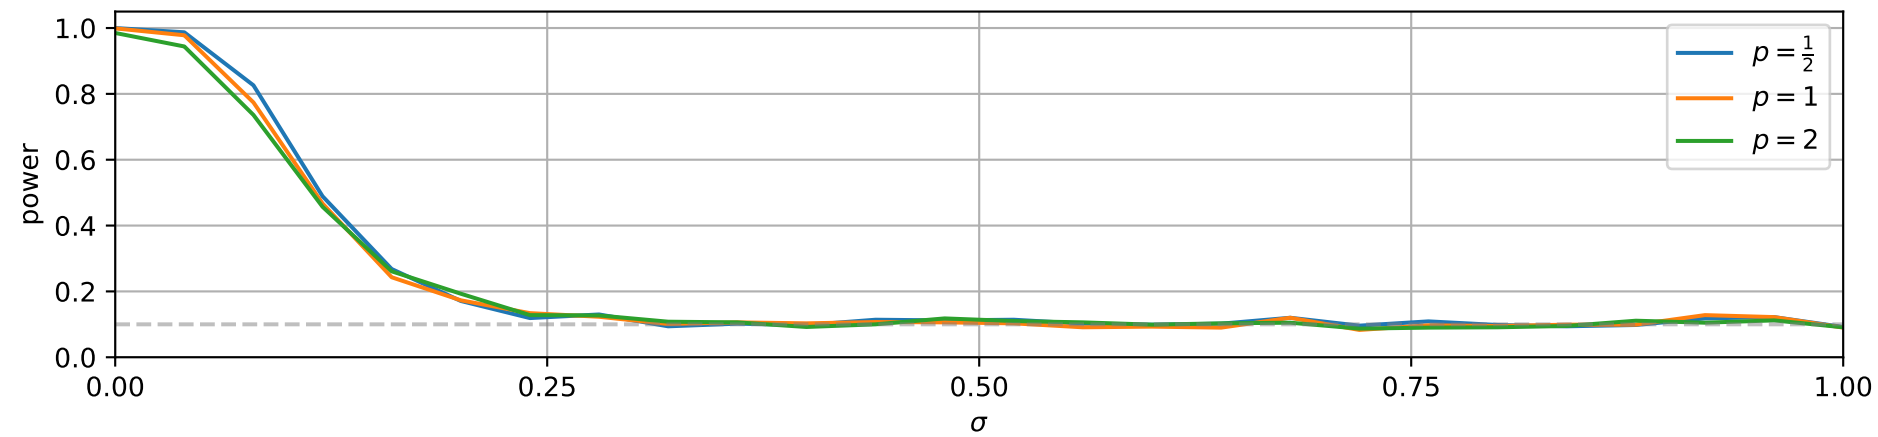

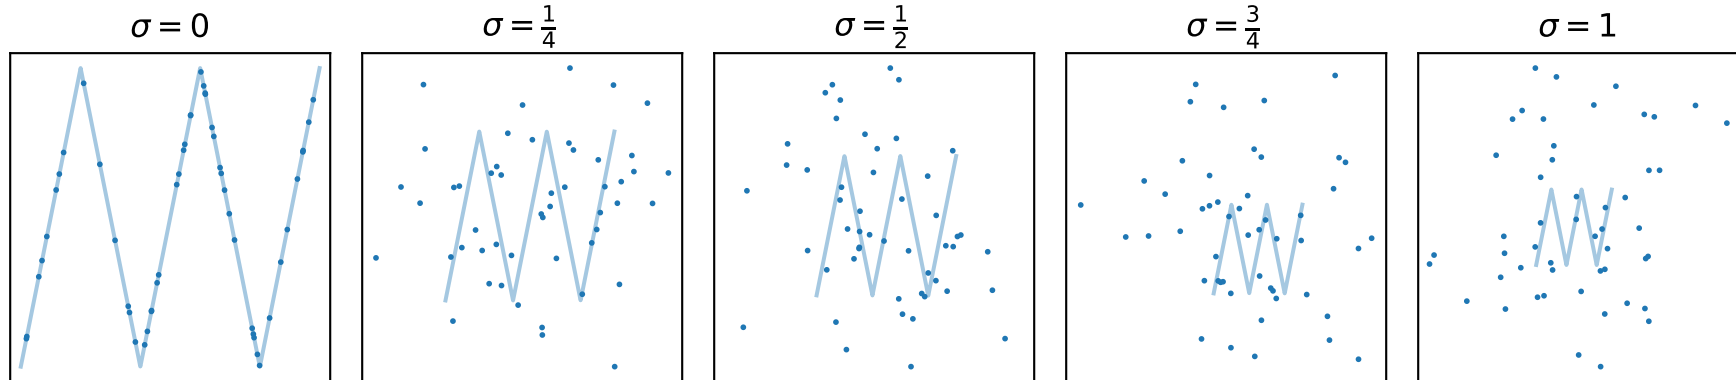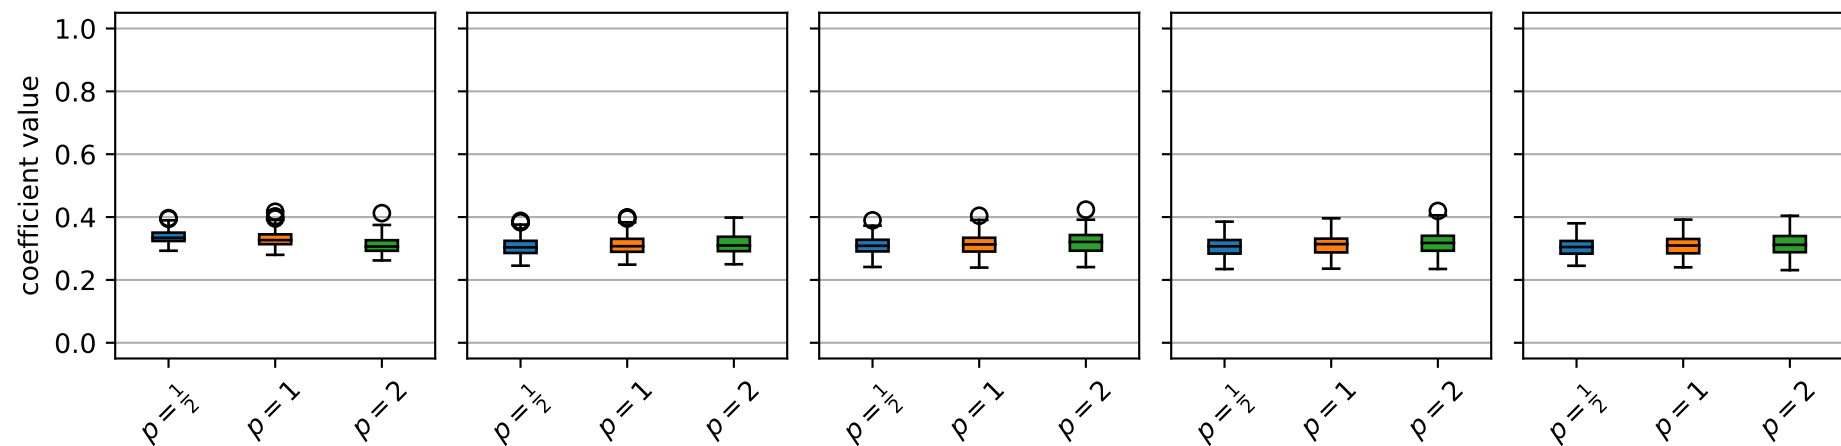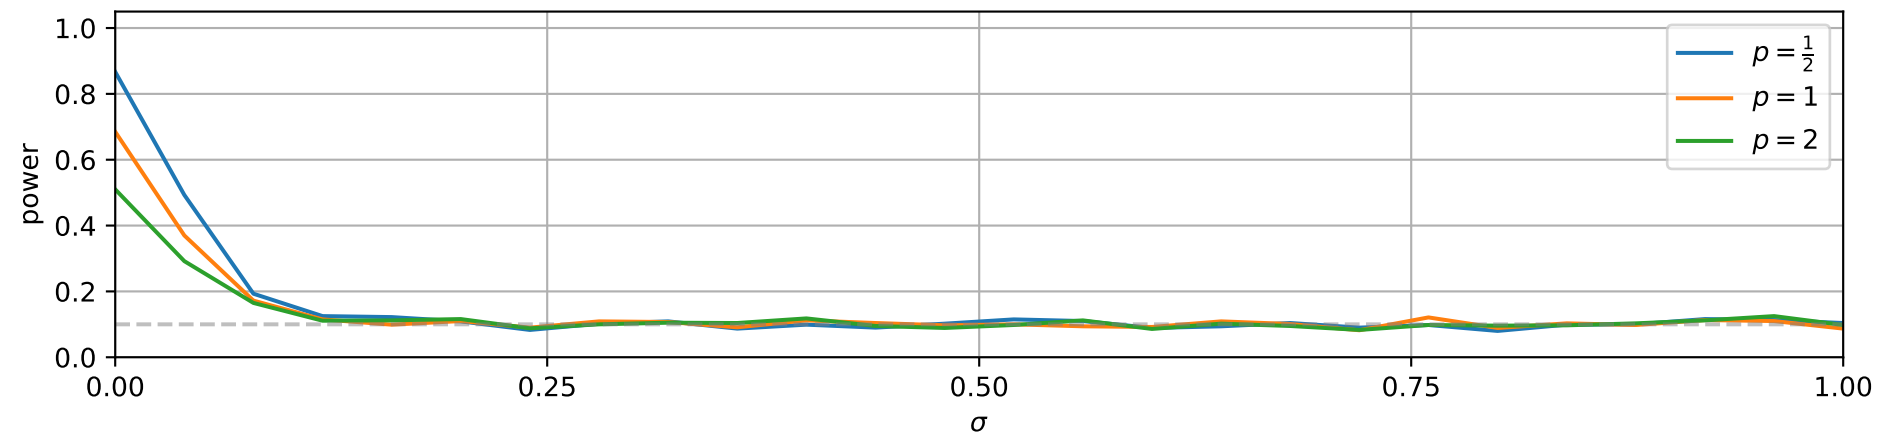

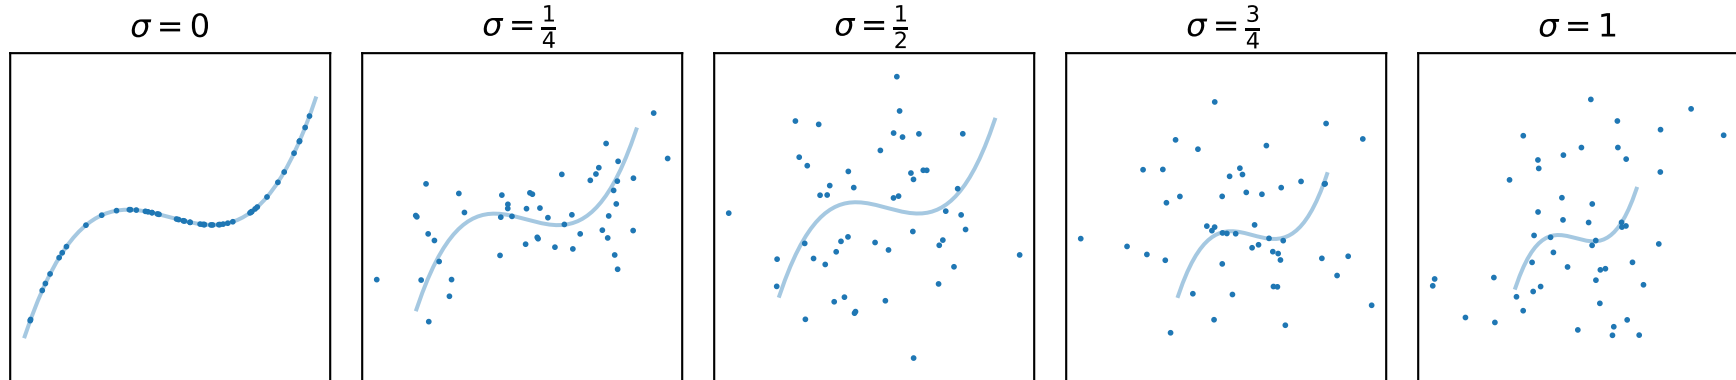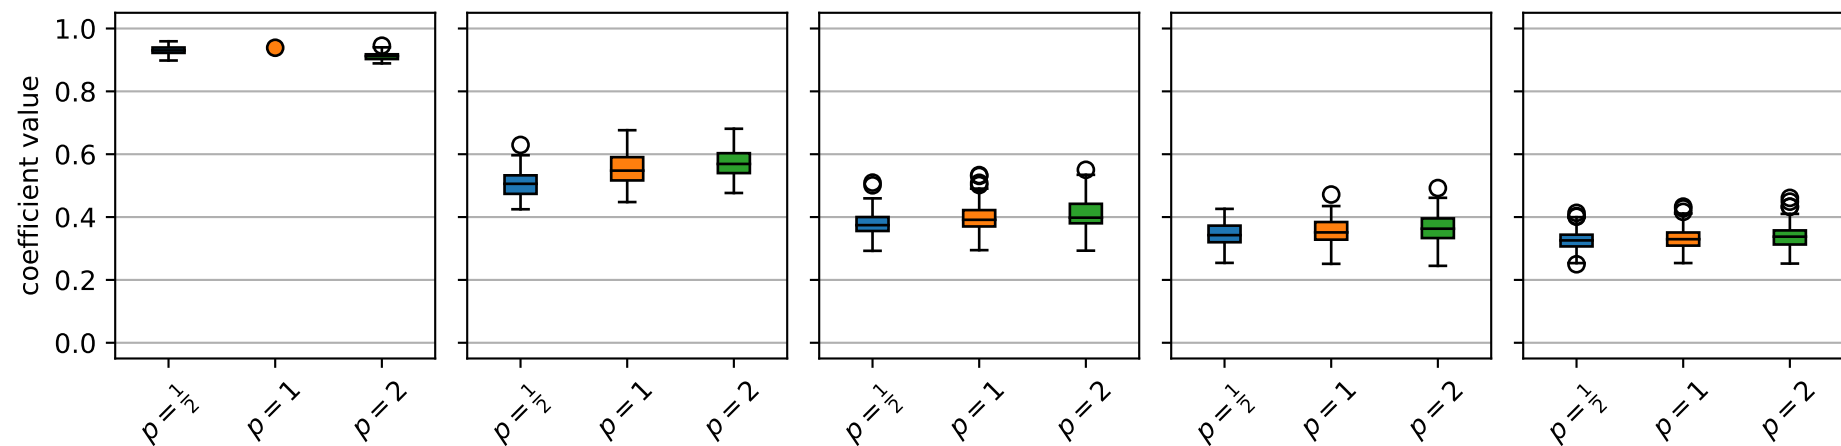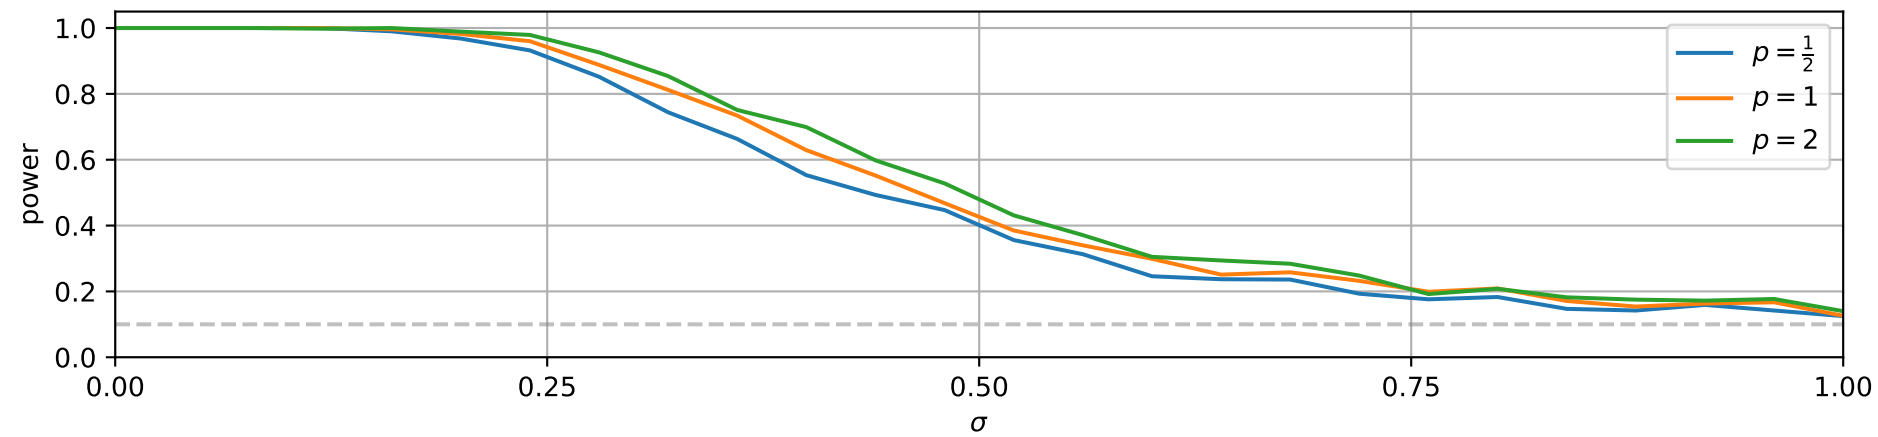

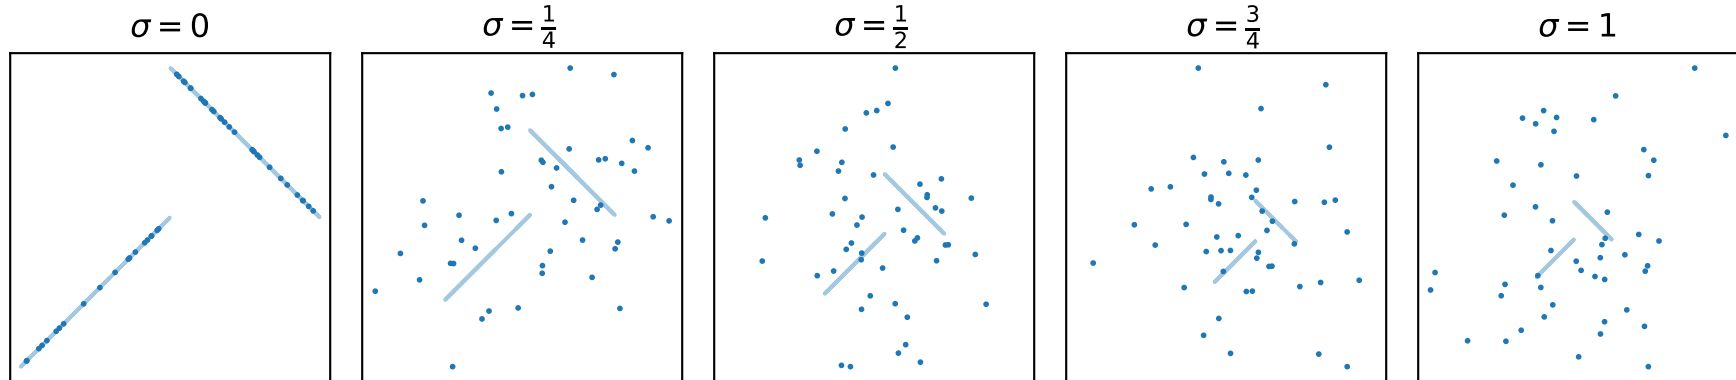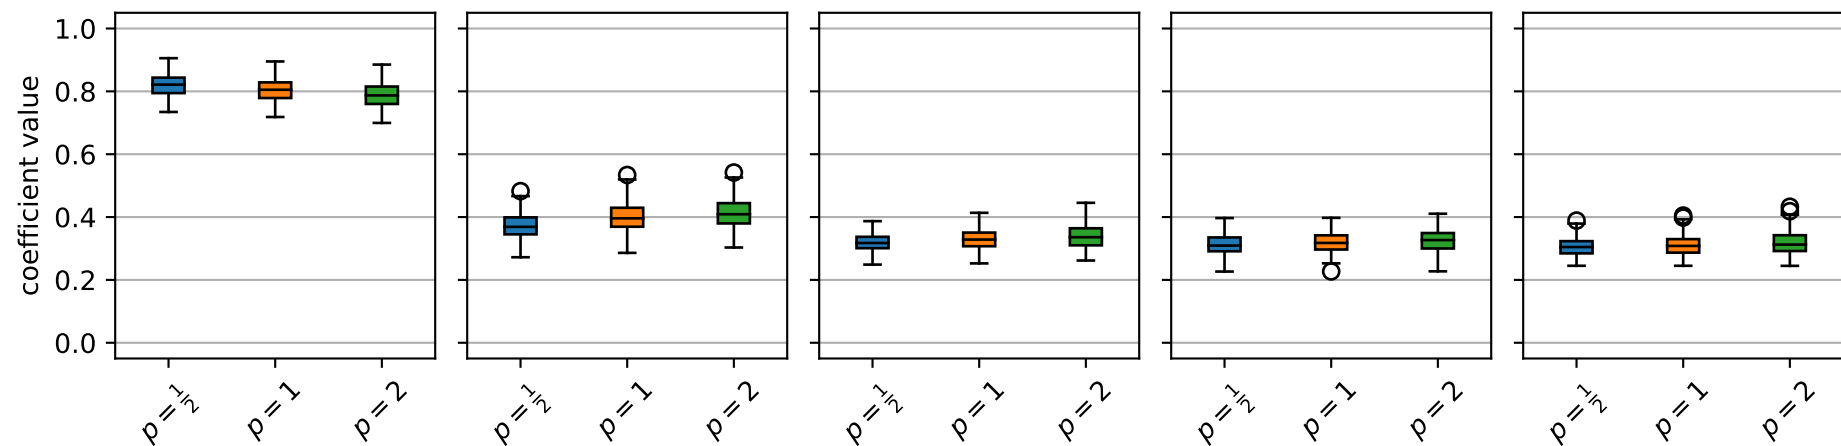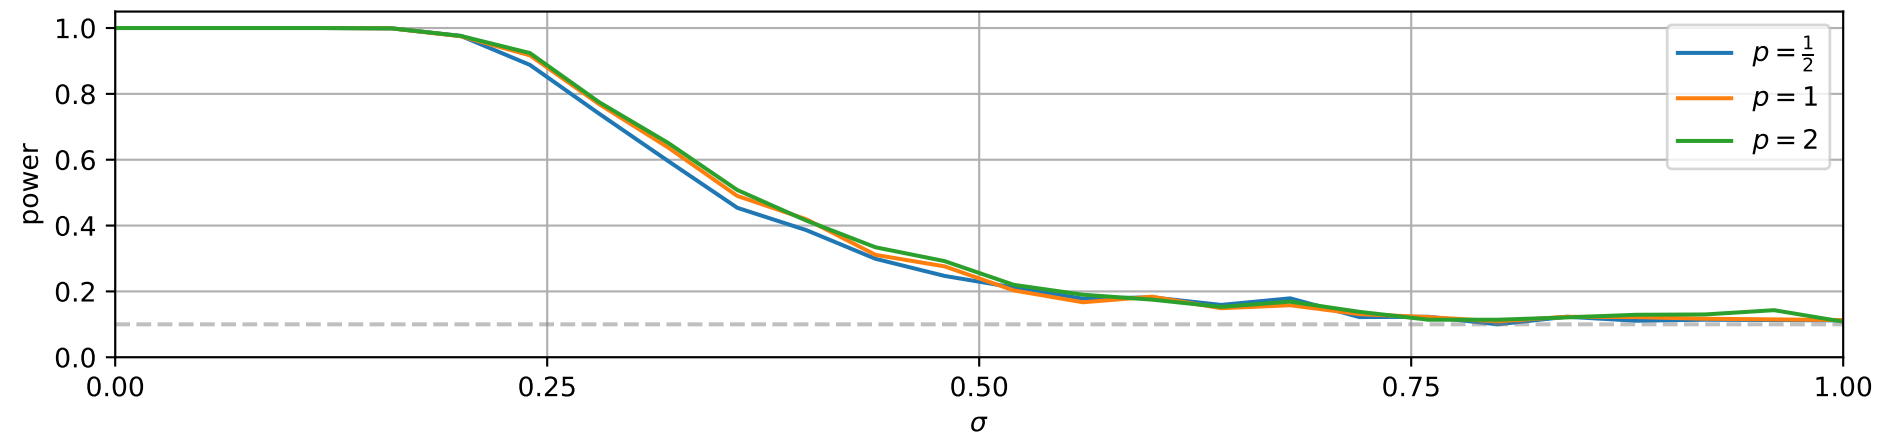

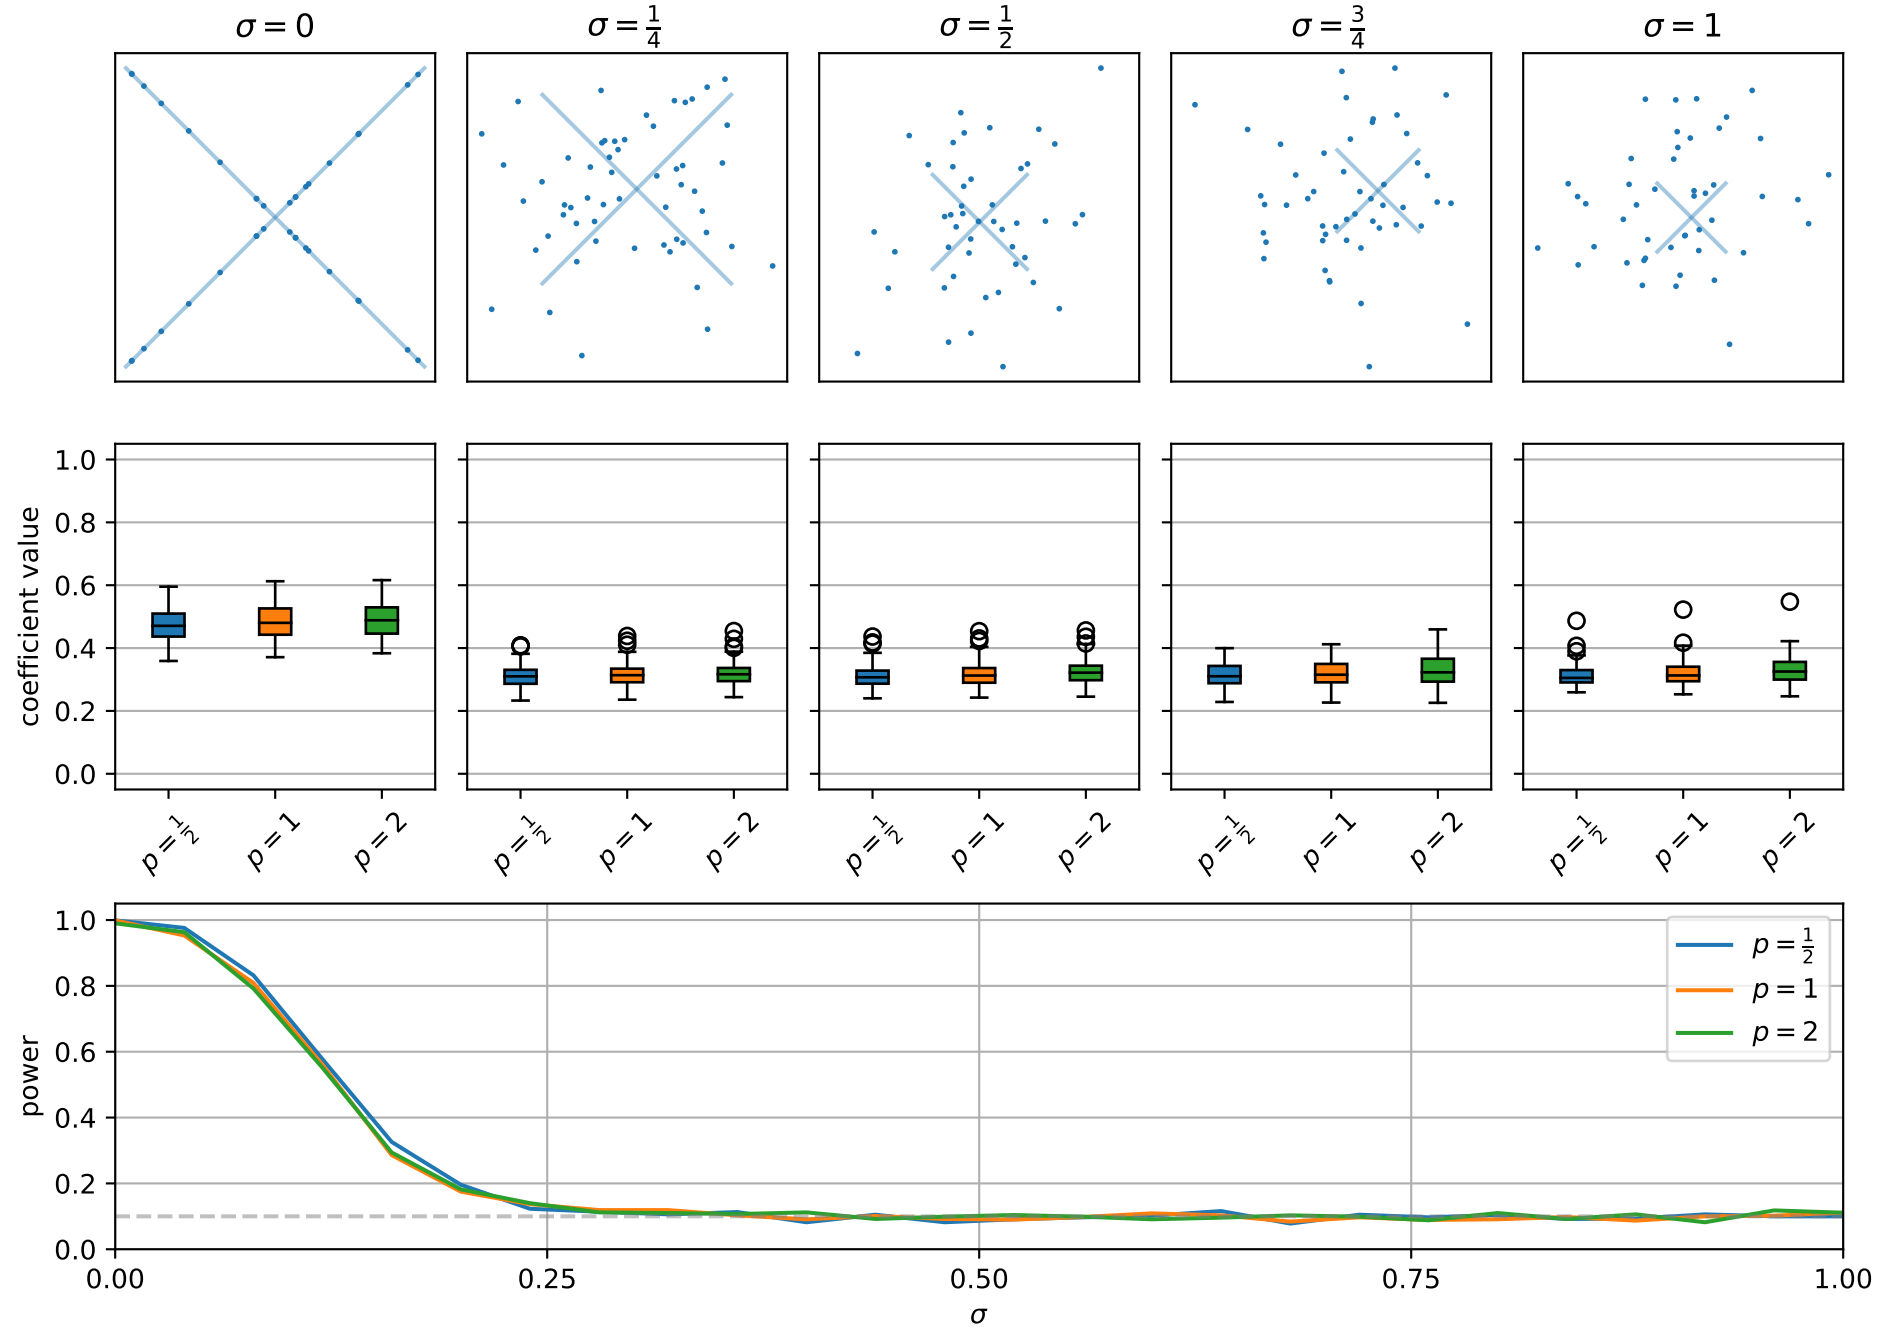

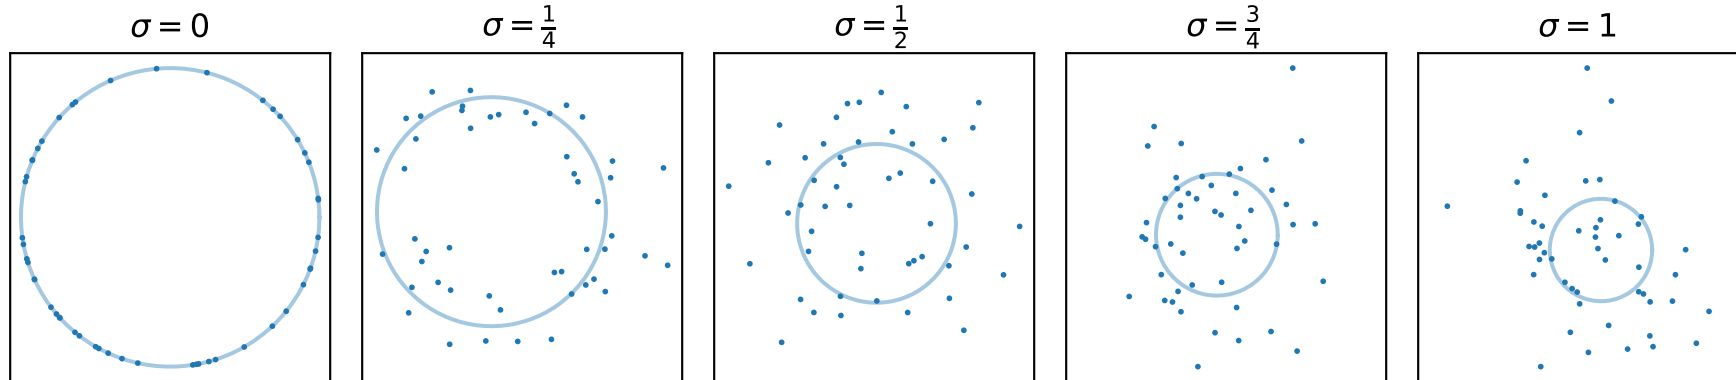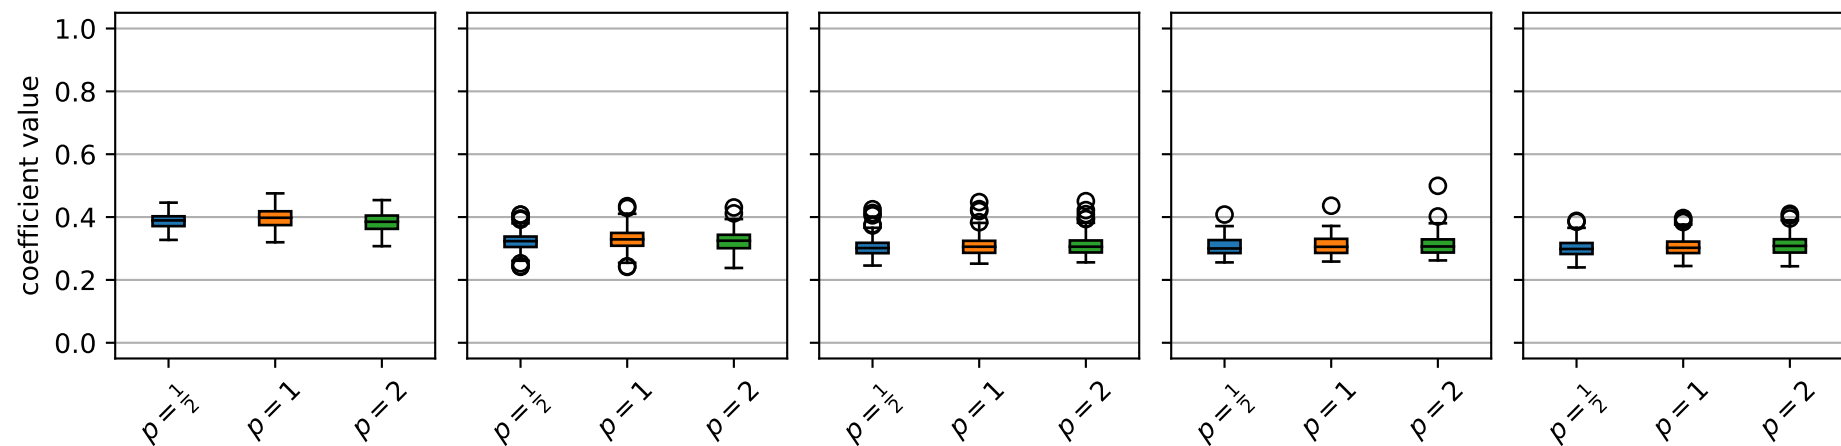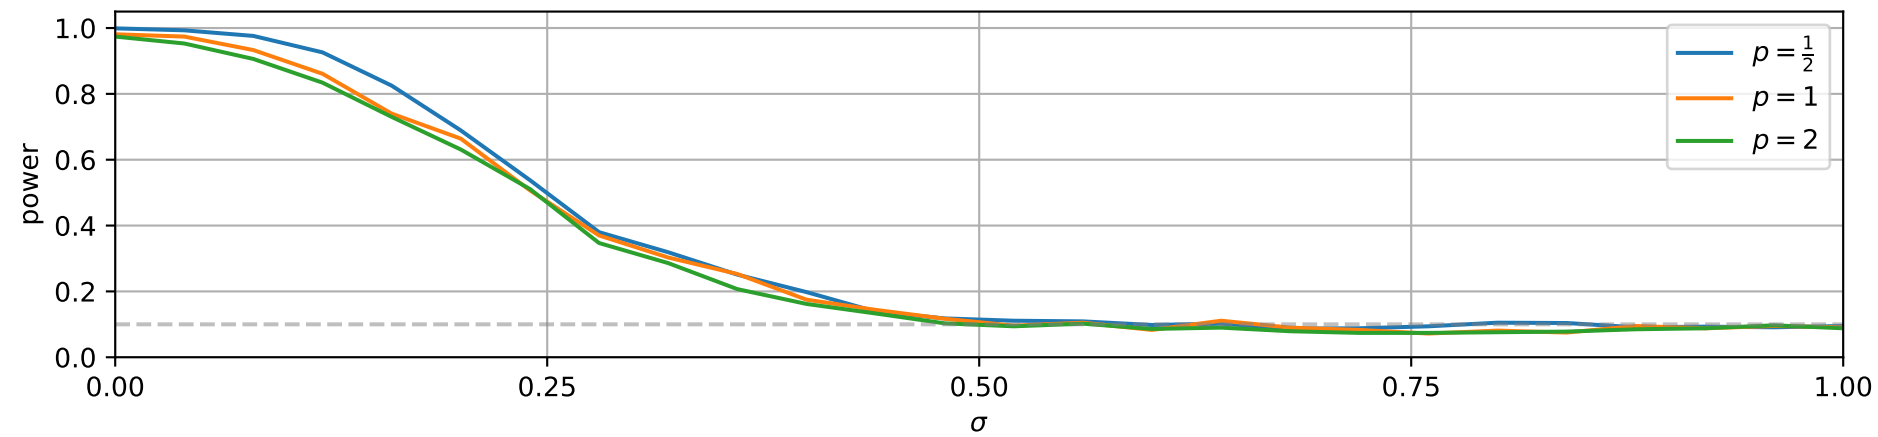



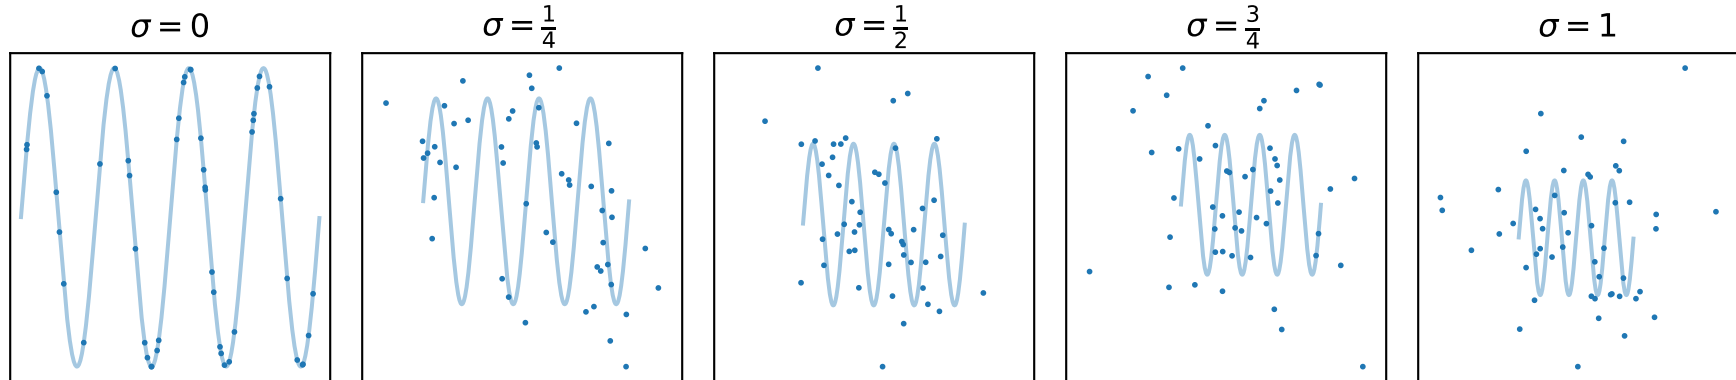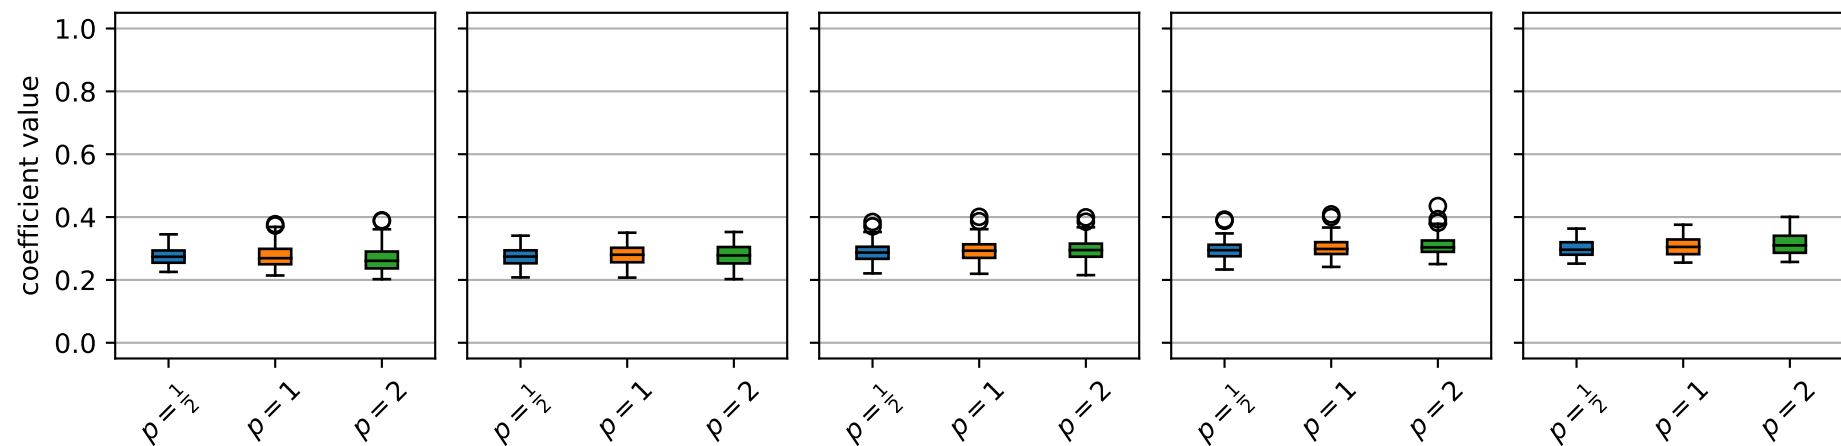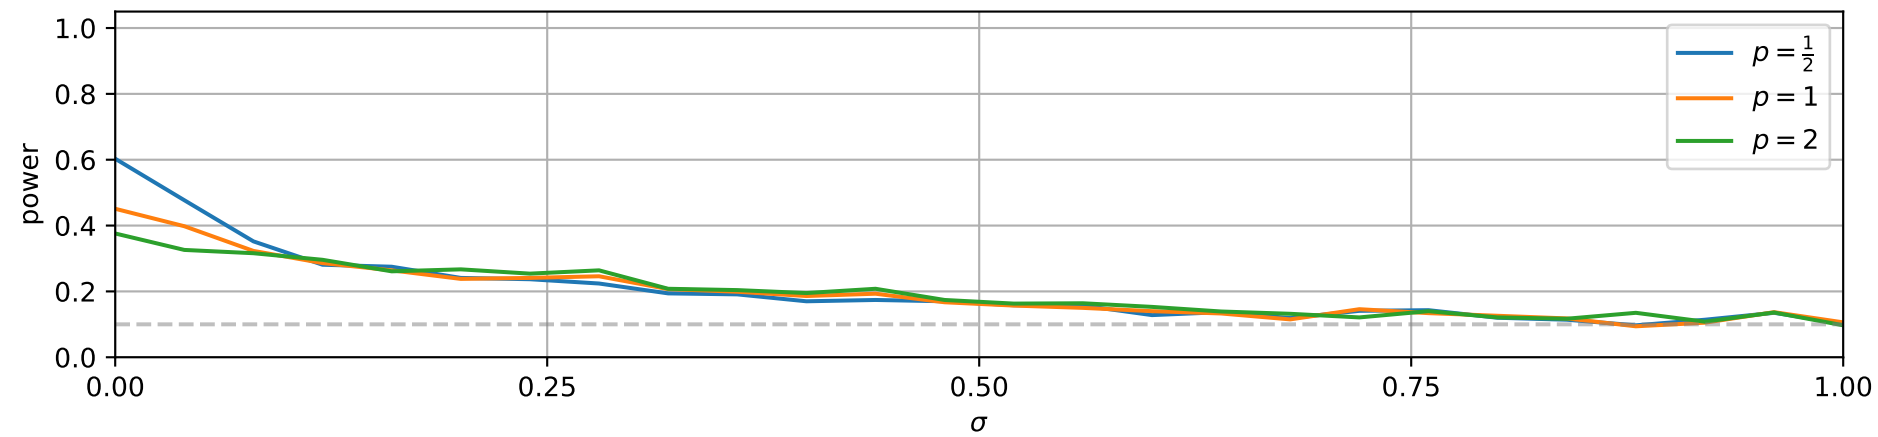

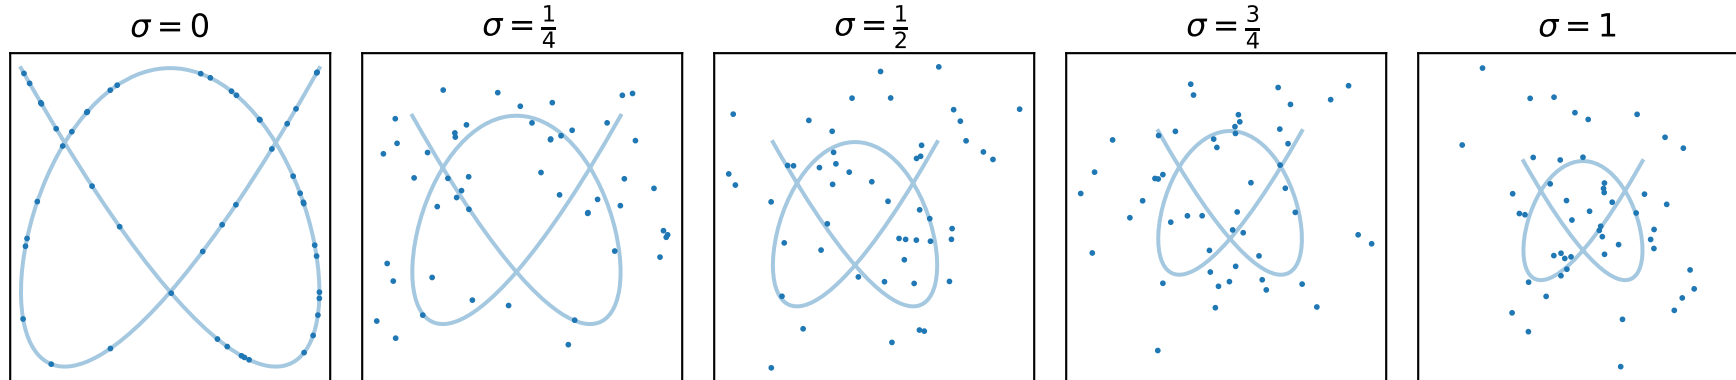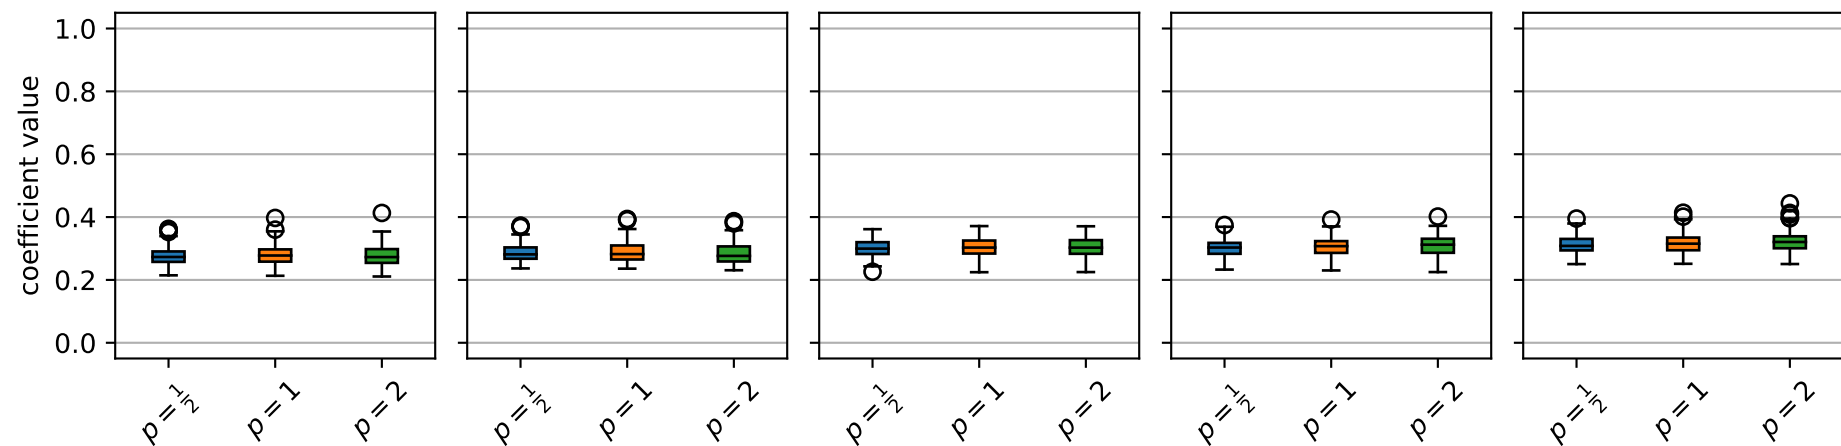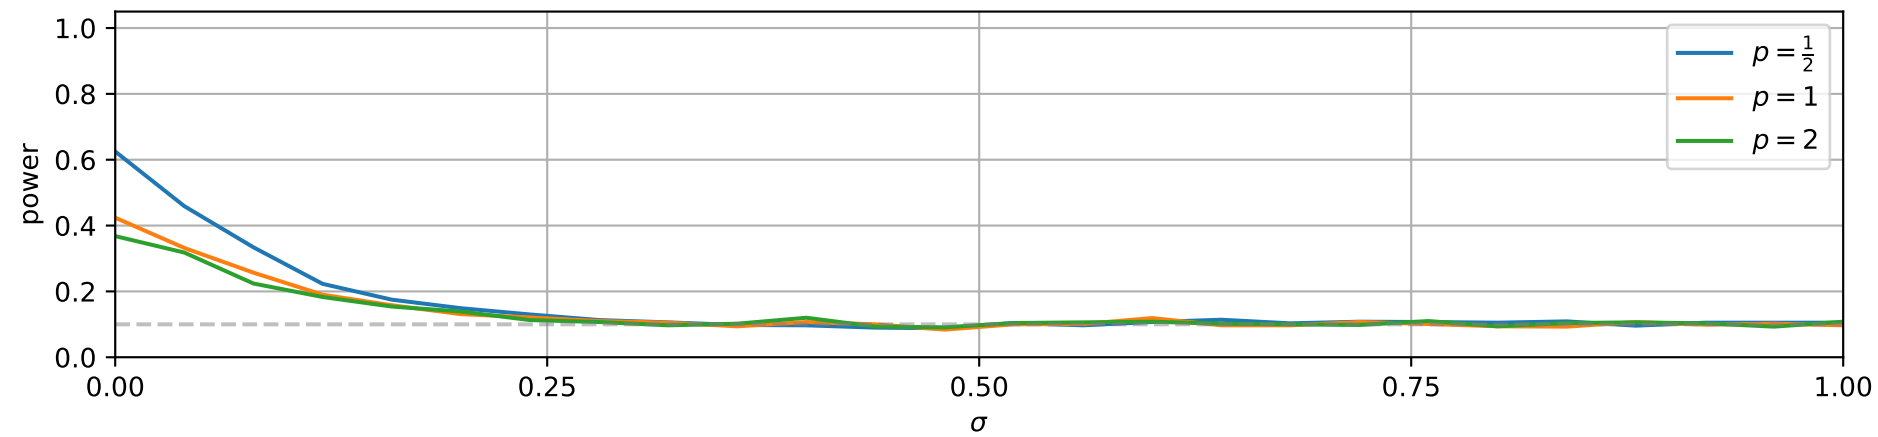

Supplement: Supplementary file 1 [file all.pdf]
